# Supplementary material for: The geography of novel and atypical research
Source: arXiv:2510.20827 source file (2025-10-09)
Supplement: Supplementary file 1 [file NoveltyCountry_SI.pdf]

# Supporting Information for
# The geography of novel and atypical research

Qing Ke[a], Tianxing Pan[b], Jin Mao[c]

[a]*School of Data Science, City University of Hong Kong, Hong Kong, China*
[b]*School of Information Management, Nanjing University, Nanjing, Jiangsu Province, China*
[c]*Center for Studies of Information Resources, Wuhan University, Wuhan, Hubei Province, China*

## S1. Language identification of MAG papers

We attempt to identify the language used by each paper in the citation network $D$. First, we rely on the citation context file from MAG, which provides the sentences where citations are made. Those citation context sentences are a reliable source of information for language detection, as they are excerpts from full-text of papers. We can detect languages for $7,256,397$ (12.9%) papers through this step. We then query the Crossref using DOIs associated with MAG papers and obtain the language information for another $37,729,909$ (67.2%) papers. Given that Crossref data are deposited by publishers, we consider the language information returned from Crossref as valid. After these two steps, we are not aware of other methods that can allow us to reliably recognize the languages of the remaining papers in a systematic manner. Note that detecting languages based on paper abstracts is only partially reliable, because our preliminary, case-based inquiry indicates that papers published in non-English journals may still have English abstracts in the MAG due to the fact that those papers have English version abstracts in addition to the original language version. We nevertheless perform language detection for the remaining papers but use the results only when the identified language is non-English, helping us cover additional $485,157$ (0.865%) papers. Doing so also means that we under-estimate the percentage of English papers, as we may have ignored genuine English papers. Yet, we improve the coverage of non-English papers, enabling us for a more accurate understanding of whether novelty/atypicality is shaped by non-English literature. Finally, considering the rise of China in science publishing, we specifically implement the identification of Chinese papers. This is done by looking at (1) if the DOI of a paper contains some particular patterns (*e.g.*, “j.cnki.” and “j.issn.”); or (2) if it is published in a list of Chinese journals whose names or publisher names correspond to the Pinyin Romanization of Chinese characters [*e.g.*, “Zhonghua Wai Ke Za Zhi” is the Pinyin Romanization of “中华外科杂志” (*Chinese Journal of Surgery*)]. We pinpoint extra $126,974$ (0.226%) papers through

this procedure. Combining all the efforts described above, we are able to identify the languages for 81.3% papers, and Table S1 lists the number of papers by language.

### S2. Supporting figures

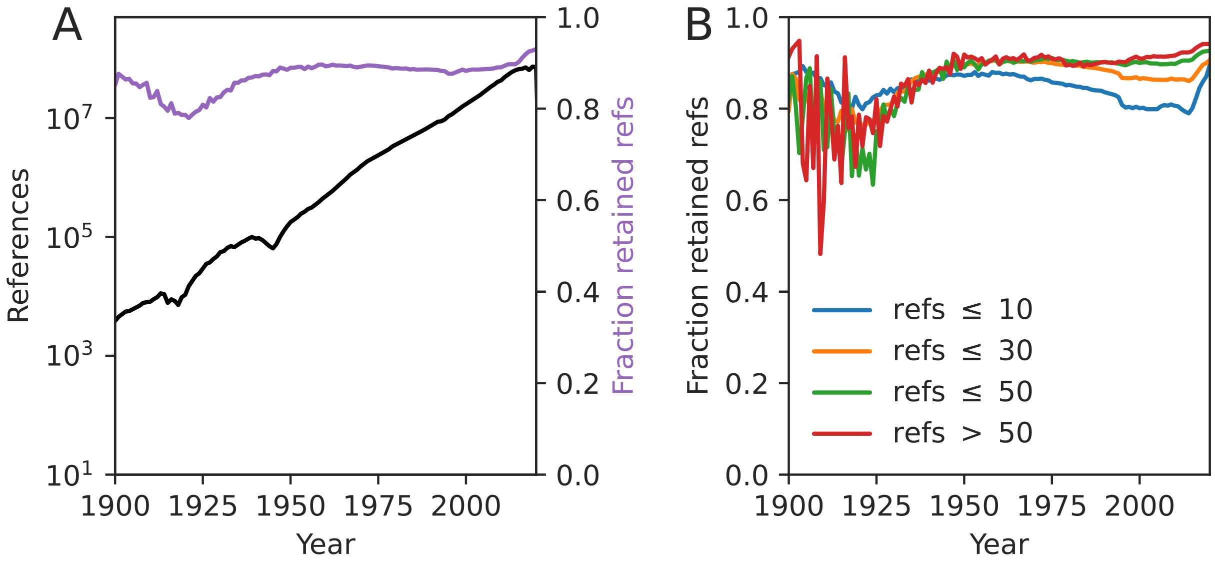


Figure S1: Statistics about cited references for the papers in our sample. (A) Total number of references (left axis) and fraction of within-sample references (right axis); (B) Fractions of within-sample references for papers grouped by their reference count.

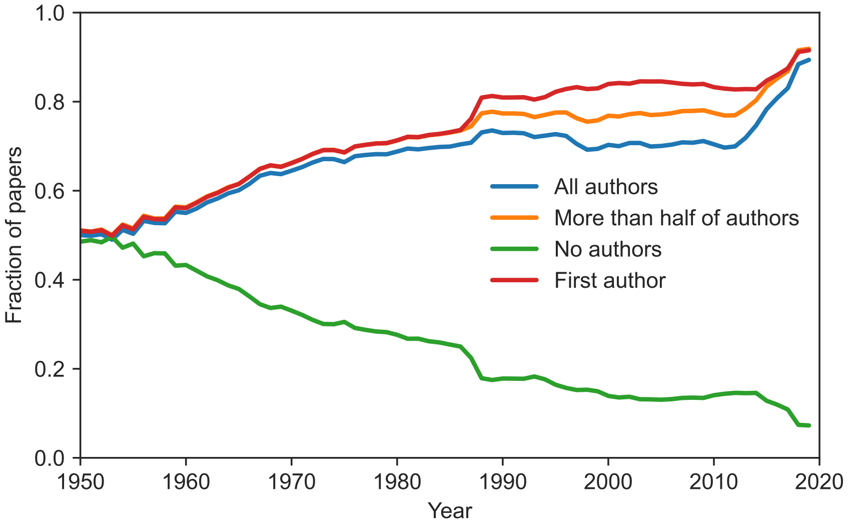


Figure S2: Paper-level statistics about the availability of author country. We present four cases: the fraction of papers where (1) all authors', (2) at least half of authors', (3) no authors', and (4) first author's country information can be extracted from their affiliation.

## S3. Supporting tables

Table S1: Number of papers by language.

| Language | Papers in $D$ Count | % | Papers in 1990–2019 Count | % |
|---|---|---|---|---|
| English | 43553148 | 77.64 | 23529936 | 90.12 |
| Unknown | 10499987 | 18.72 | 2089721 | 8.003 |
| German | 826810 | 1.474 | 95054 | 0.3640 |
| French | 446279 | 0.7955 | 125423 | 0.4804 |
| Spanish | 232403 | 0.4143 | 122302 | 0.4684 |
| Chinese | 134262 | 0.2393 | 4518 | 0.0173 |
| Portuguese | 123814 | 0.2207 | 60086 | 0.2301 |
| Japanese | 95168 | 0.1696 | 17504 | 0.0670 |
| Korean | 63749 | 0.1136 | 33490 | 0.1283 |
| Italian | 18556 | 0.0331 | 4744 | 0.0182 |
| Dutch | 17825 | 0.0318 | 3061 | 0.0117 |

Table S2: Total number papers by category and decade.

| Period | All papers Count | All papers with affiliation | Novel papers Count | Novel papers with affiliation | Atypical papers Count | Atypical papers with affiliation |
|---|---|---|---|---|---|---|
| 1990–2019 | 26110499 | 25461110.87 | 9876914 | 9636678.09 | 2087506 | 2041285.11 |
| 1990s | 3794436 | 3693919.18 | 1355976 | 1321308.86 | 271002 | 264324.98 |
| 2000s | 7577519 | 7329372.20 | 2721957 | 2631367.18 | 551673 | 534314.46 |
| 2010s | 14738544 | 14437819.49 | 5798981 | 5684002.05 | 1264831 | 1242645.67 |

Table S3: Statistics about the production of science and novel and atypical science in the 1990s for a list of 38 countries/regions.

| | All papers | | Novel papers | | | | Atypical papers | | | |
|---|---|---|---|---|---|---|---|---|---|---|
| Country/region | Count | % | Count | % | $r_N$ | $p$-val | Count | % | $r_A$ | $p$-val |
| US | 1306684.88 | 35.37 | 482828.33 | 36.54 | 1.03 | *** | 100087.59 | 37.87 | 1.07 | *** |
| UK | 323982.77 | 8.77 | 114837.90 | 8.69 | 0.99 | *** | 19703.72 | 7.45 | 0.85 | *** |
| Japan | 320355.48 | 8.67 | 122328.44 | 9.26 | 1.07 | *** | 25324.19 | 9.58 | 1.10 | *** |
| Germany | 222115.16 | 6.01 | 78863.14 | 5.97 | 0.99 | ** | 16607.61 | 6.28 | 1.04 | *** |
| France | 170676.18 | 4.62 | 62006.72 | 4.69 | 1.02 | *** | 12945.79 | 4.90 | 1.06 | *** |
| Canada | 144307.38 | 3.91 | 51338.34 | 3.89 | 0.99 | | 9979.55 | 3.78 | 0.97 | *** |
| Italy | 115316.14 | 3.12 | 41549.28 | 3.14 | 1.01 | * | 8500.91 | 3.22 | 1.03 | ** |
| Australia | 95941.15 | 2.60 | 32145.92 | 2.43 | 0.94 | *** | 5617.68 | 2.13 | 0.82 | *** |
| Netherlands | 81059.44 | 2.19 | 31005.37 | 2.35 | 1.07 | *** | 5915.64 | 2.24 | 1.02 | |
| Spain | 74144.01 | 2.01 | 24800.65 | 1.88 | 0.94 | *** | 5702.48 | 2.16 | 1.07 | *** |
| India | 68871.38 | 1.86 | 23879.91 | 1.81 | 0.97 | *** | 4542.99 | 1.72 | 0.92 | *** |
| Sweden | 62120.83 | 1.68 | 26608.05 | 2.01 | 1.20 | *** | 4442.05 | 1.68 | 1.00 | |
| Russia | 56351.27 | 1.53 | 14628.08 | 1.11 | 0.73 | *** | 3144.21 | 1.19 | 0.78 | *** |
| China | 44817.81 | 1.21 | 11395.94 | 0.86 | 0.71 | *** | 2986.55 | 1.13 | 0.93 | *** |
| Switzerland | 43067.97 | 1.17 | 15810.26 | 1.20 | 1.03 | *** | 3603.96 | 1.36 | 1.17 | *** |
| Israel | 38412.32 | 1.04 | 13719.04 | 1.04 | 1.00 | | 2540.88 | 0.96 | 0.92 | *** |
| Taiwan | 37474.26 | 1.01 | 10600.66 | 0.80 | 0.79 | *** | 2622.36 | 0.99 | 0.98 | |
| Belgium | 34413.64 | 0.93 | 12758.83 | 0.97 | 1.04 | *** | 2492.93 | 0.94 | 1.01 | |
| Brazil | 29950.85 | 0.81 | 10351.00 | 0.78 | 0.97 | *** | 1792.39 | 0.68 | 0.84 | *** |
| Korea | 29093.31 | 0.79 | 7964.68 | 0.60 | 0.77 | *** | 2034.75 | 0.77 | 0.98 | |
| Denmark | 28585.41 | 0.77 | 11283.79 | 0.85 | 1.10 | *** | 1996.70 | 0.76 | 0.98 | |
| Finland | 28059.08 | 0.76 | 11352.19 | 0.86 | 1.13 | *** | 1896.44 | 0.72 | 0.94 | ** |
| Poland | 26422.73 | 0.72 | 7821.02 | 0.59 | 0.83 | *** | 1450.06 | 0.55 | 0.77 | *** |
| Austria | 21703.36 | 0.59 | 8227.24 | 0.62 | 1.06 | *** | 1592.17 | 0.60 | 1.03 | |
| Norway | 20205.78 | 0.55 | 7897.78 | 0.60 | 1.09 | *** | 1286.18 | 0.49 | 0.89 | *** |
| South Africa | 18207.41 | 0.49 | 5182.10 | 0.39 | 0.80 | *** | 878.05 | 0.33 | 0.67 | *** |
| New Zealand | 16510.31 | 0.45 | 5749.82 | 0.44 | 0.97 | ** | 1004.74 | 0.38 | 0.85 | *** |
| Greece | 15301.35 | 0.41 | 4709.28 | 0.36 | 0.86 | *** | 1033.43 | 0.39 | 0.94 | * |
| Mexico | 15215.60 | 0.41 | 5640.96 | 0.43 | 1.04 | *** | 1121.05 | 0.42 | 1.03 | |
| Turkey | 14074.29 | 0.38 | 4541.51 | 0.34 | 0.90 | *** | 733.79 | 0.28 | 0.73 | *** |
| Hong Kong | 13803.29 | 0.37 | 3531.30 | 0.27 | 0.72 | *** | 722.56 | 0.27 | 0.73 | *** |
| Hungary | 12948.53 | 0.35 | 4344.41 | 0.33 | 0.94 | *** | 913.56 | 0.35 | 0.99 | |
| Czechia | 12841.54 | 0.35 | 4114.29 | 0.31 | 0.90 | *** | 684.98 | 0.26 | 0.75 | *** |
| Singapore | 10434.00 | 0.28 | 2506.42 | 0.19 | 0.67 | *** | 516.41 | 0.20 | 0.69 | *** |
| Egypt | 9646.99 | 0.26 | 3492.44 | 0.26 | 1.01 | | 557.41 | 0.21 | 0.81 | *** |
| Portugal | 8054.62 | 0.22 | 2477.75 | 0.19 | 0.86 | *** | 568.03 | 0.21 | 0.99 | |
| Malaysia | 3226.39 | 0.09 | 976.13 | 0.07 | 0.85 | *** | 177.16 | 0.07 | 0.77 | *** |
| Iran | 2189.15 | 0.06 | 562.50 | 0.04 | 0.72 | *** | 133.31 | 0.05 | 0.85 | * |
| *Total* | 3576586.08 | 96.82 | 1283831.50 | 97.16 | – | – | 257854.25 | 97.55 | – | – |

* $p < 0.05$, ** $p < 0.01$, *** $p < 0.001$

Table S4: Statistics about the production of science and novel and atypical science in the 2000s for a list of 38 countries/regions.

| | All papers | | Novel papers | | | | Atypical papers | | | |
|---|---|---|---|---|---|---|---|---|---|---|
| Country/region | Count | % | Count | % | $r_N$ | $p$-val | Count | % | $r_A$ | $p$-val |
| US | 2210910.02 | 30.17 | 828471.29 | 31.48 | 1.04 | *** | 175276.29 | 32.80 | 1.09 | *** |
| UK | 544982.78 | 7.44 | 189343.39 | 7.20 | 0.97 | *** | 34279.00 | 6.42 | 0.86 | *** |
| Japan | 511276.42 | 6.98 | 191558.00 | 7.28 | 1.04 | *** | 41802.04 | 7.82 | 1.12 | *** |
| Germany | 379849.63 | 5.18 | 138701.01 | 5.27 | 1.02 | *** | 30679.49 | 5.74 | 1.11 | *** |
| China | 328453.61 | 4.48 | 113303.40 | 4.31 | 0.96 | *** | 27158.88 | 5.08 | 1.13 | *** |
| France | 291650.71 | 3.98 | 102278.65 | 3.89 | 0.98 | *** | 21982.00 | 4.11 | 1.03 | *** |
| Canada | 253401.64 | 3.46 | 88384.48 | 3.36 | 0.97 | *** | 16983.99 | 3.18 | 0.92 | *** |
| Italy | 230387.11 | 3.14 | 84596.25 | 3.21 | 1.02 | *** | 17614.13 | 3.30 | 1.05 | *** |
| Spain | 202024.64 | 2.76 | 63866.30 | 2.43 | 0.88 | *** | 14170.50 | 2.65 | 0.96 | *** |
| Australia | 199417.96 | 2.72 | 67161.13 | 2.55 | 0.94 | *** | 11561.65 | 2.16 | 0.80 | *** |
| India | 162755.91 | 2.22 | 59298.12 | 2.25 | 1.01 | *** | 11882.37 | 2.22 | 1.00 | |
| Korea | 157293.70 | 2.15 | 55330.13 | 2.10 | 0.98 | *** | 11706.53 | 2.19 | 1.02 | ** |
| Brazil | 151378.77 | 2.07 | 56586.39 | 2.15 | 1.04 | *** | 8461.77 | 1.58 | 0.77 | *** |
| Netherlands | 131638.18 | 1.80 | 50464.73 | 1.92 | 1.07 | *** | 10078.02 | 1.89 | 1.05 | *** |
| Russia | 127004.54 | 1.73 | 33766.74 | 1.28 | 0.74 | *** | 6802.48 | 1.27 | 0.73 | *** |
| Taiwan | 104777.46 | 1.43 | 35739.59 | 1.36 | 0.95 | *** | 7528.47 | 1.41 | 0.99 | |
| Sweden | 102795.21 | 1.40 | 41728.37 | 1.59 | 1.13 | *** | 7250.45 | 1.36 | 0.97 | ** |
| Turkey | 80361.29 | 1.10 | 28270.32 | 1.07 | 0.98 | *** | 4325.21 | 0.81 | 0.74 | *** |
| Switzerland | 75812.00 | 1.03 | 28335.57 | 1.08 | 1.04 | *** | 6333.12 | 1.19 | 1.15 | *** |
| Belgium | 67622.42 | 0.92 | 24161.55 | 0.92 | 1.00 | | 5255.95 | 0.98 | 1.07 | *** |
| Poland | 63710.23 | 0.87 | 21197.51 | 0.81 | 0.93 | *** | 3766.30 | 0.70 | 0.81 | *** |
| Israel | 62444.14 | 0.85 | 23421.54 | 0.89 | 1.04 | *** | 4354.10 | 0.81 | 0.96 | ** |
| Denmark | 54705.29 | 0.75 | 21970.24 | 0.83 | 1.12 | *** | 4115.87 | 0.77 | 1.03 | * |
| Finland | 50045.13 | 0.68 | 19162.83 | 0.73 | 1.07 | *** | 3578.95 | 0.67 | 0.98 | |
| Greece | 45464.20 | 0.62 | 15315.59 | 0.58 | 0.94 | *** | 2883.38 | 0.54 | 0.87 | *** |
| Mexico | 45443.31 | 0.62 | 16197.35 | 0.62 | 0.99 | | 3023.61 | 0.57 | 0.91 | *** |
| Hong Kong | 43437.42 | 0.59 | 13309.50 | 0.51 | 0.85 | *** | 2750.24 | 0.51 | 0.87 | *** |
| Austria | 43362.84 | 0.59 | 16346.23 | 0.62 | 1.05 | *** | 3200.21 | 0.60 | 1.01 | |
| Norway | 40986.68 | 0.56 | 15155.63 | 0.58 | 1.03 | *** | 2513.36 | 0.47 | 0.84 | *** |
| Iran | 40055.69 | 0.55 | 12482.86 | 0.47 | 0.87 | *** | 2731.65 | 0.51 | 0.94 | *** |
| South Africa | 34720.86 | 0.47 | 10844.99 | 0.41 | 0.87 | *** | 1625.98 | 0.30 | 0.64 | *** |
| Singapore | 34106.88 | 0.47 | 10562.07 | 0.40 | 0.86 | *** | 2303.75 | 0.43 | 0.93 | *** |
| New Zealand | 33918.63 | 0.46 | 11545.36 | 0.44 | 0.95 | *** | 1994.40 | 0.37 | 0.81 | *** |
| Portugal | 31112.36 | 0.42 | 10338.13 | 0.39 | 0.93 | *** | 1970.35 | 0.37 | 0.87 | *** |
| Czechia | 26673.92 | 0.36 | 8980.45 | 0.34 | 0.94 | *** | 1649.86 | 0.31 | 0.85 | *** |
| Hungary | 26518.41 | 0.36 | 9726.86 | 0.37 | 1.02 | ** | 1784.43 | 0.33 | 0.92 | *** |
| Egypt | 19730.25 | 0.27 | 7303.27 | 0.28 | 1.03 | *** | 1217.99 | 0.23 | 0.85 | *** |
| Malaysia | 13835.37 | 0.19 | 4084.72 | 0.16 | 0.82 | *** | 694.65 | 0.13 | 0.69 | *** |
| *Total* | 7024065.59 | 95.83 | 2529290.56 | 96.12 | – | – | 517291.40 | 96.81 | – | – |

* $p < 0.05$, ** $p < 0.01$, *** $p < 0.001$

Table S5: Statistics about the production of science and novel and atypical science in the 2010s for a list of 38 countries/regions.

| | All papers | | Novel papers | | | | Atypical papers | | | |
|---|---|---|---|---|---|---|---|---|---|---|
| Country/region | Count | % | Count | % | $r_N$ | $p$-val | Count | % | $r_A$ | $p$-val |
| US | 3415093.38 | 23.65 | 1351529.33 | 23.78 | 1.01 | *** | 319261.48 | 25.69 | 1.09 | *** |
| China | 1840141.69 | 12.75 | 743641.64 | 13.08 | 1.03 | *** | 202336.66 | 16.28 | 1.28 | *** |
| UK | 795888.17 | 5.51 | 302753.17 | 5.33 | 0.97 | *** | 60818.41 | 4.89 | 0.89 | *** |
| Germany | 619673.43 | 4.29 | 235081.55 | 4.14 | 0.96 | *** | 59347.28 | 4.78 | 1.11 | *** |
| Japan | 619416.49 | 4.29 | 230861.69 | 4.06 | 0.95 | *** | 56541.48 | 4.55 | 1.06 | *** |
| India | 530854.59 | 3.68 | 219162.26 | 3.86 | 1.05 | *** | 44148.43 | 3.55 | 0.97 | *** |
| Canada | 441892.38 | 3.06 | 169679.71 | 2.99 | 0.98 | *** | 35539.99 | 2.86 | 0.93 | *** |
| France | 439334.72 | 3.04 | 163185.11 | 2.87 | 0.94 | *** | 40769.25 | 3.28 | 1.08 | *** |
| Korea | 432264.28 | 2.99 | 176181.89 | 3.10 | 1.04 | *** | 37776.77 | 3.04 | 1.02 | *** |
| Italy | 416771.13 | 2.89 | 164485.34 | 2.89 | 1.00 | | 32579.37 | 2.62 | 0.91 | *** |
| Australia | 415258.97 | 2.88 | 159756.36 | 2.81 | 0.98 | *** | 28992.25 | 2.33 | 0.81 | *** |
| Spain | 384478.50 | 2.66 | 136838.38 | 2.41 | 0.90 | *** | 30413.63 | 2.45 | 0.92 | *** |
| Brazil | 358335.41 | 2.48 | 156405.86 | 2.75 | 1.11 | *** | 21513.19 | 1.73 | 0.70 | *** |
| Iran | 278067.33 | 1.93 | 117703.18 | 2.07 | 1.08 | *** | 20727.19 | 1.67 | 0.87 | *** |
| Russia | 234744.47 | 1.63 | 74516.94 | 1.31 | 0.81 | *** | 13439.94 | 1.08 | 0.67 | *** |
| Netherlands | 228589.41 | 1.58 | 94755.57 | 1.67 | 1.05 | *** | 20264.61 | 1.63 | 1.03 | *** |
| Taiwan | 187101.54 | 1.30 | 75308.26 | 1.32 | 1.02 | *** | 16040.93 | 1.29 | 1.00 | |
| Turkey | 175446.60 | 1.22 | 67023.83 | 1.18 | 0.97 | *** | 10767.35 | 0.87 | 0.71 | *** |
| Poland | 158797.68 | 1.10 | 63697.93 | 1.12 | 1.02 | *** | 10024.66 | 0.81 | 0.73 | *** |
| Sweden | 148780.15 | 1.03 | 59715.20 | 1.05 | 1.02 | *** | 12192.80 | 0.98 | 0.95 | *** |
| Switzerland | 137559.13 | 0.95 | 54538.53 | 0.96 | 1.01 | * | 13983.25 | 1.13 | 1.18 | *** |
| Belgium | 117214.47 | 0.81 | 45058.16 | 0.79 | 0.98 | *** | 10140.95 | 0.82 | 1.01 | |
| Mexico | 99726.91 | 0.69 | 41404.28 | 0.73 | 1.05 | *** | 6937.76 | 0.56 | 0.81 | *** |
| Denmark | 93714.12 | 0.65 | 39276.50 | 0.69 | 1.06 | *** | 8135.48 | 0.65 | 1.01 | |
| South Africa | 90212.59 | 0.62 | 34121.71 | 0.60 | 0.96 | *** | 4633.47 | 0.37 | 0.60 | *** |
| Malaysia | 87181.79 | 0.60 | 37812.97 | 0.67 | 1.10 | *** | 5527.69 | 0.44 | 0.74 | *** |
| Portugal | 86810.21 | 0.60 | 35704.79 | 0.63 | 1.04 | *** | 6470.40 | 0.52 | 0.87 | *** |
| Israel | 86373.58 | 0.60 | 32789.61 | 0.58 | 0.96 | *** | 6971.90 | 0.56 | 0.94 | *** |
| Norway | 76593.89 | 0.53 | 29180.42 | 0.51 | 0.97 | *** | 5346.54 | 0.43 | 0.81 | *** |
| Austria | 75624.86 | 0.52 | 30282.95 | 0.53 | 1.02 | *** | 6551.64 | 0.53 | 1.01 | |
| Finland | 73878.03 | 0.51 | 28947.22 | 0.51 | 1.00 | | 5965.44 | 0.48 | 0.94 | *** |
| Hong Kong | 72844.92 | 0.50 | 26741.83 | 0.47 | 0.93 | *** | 6639.28 | 0.53 | 1.06 | *** |
| Greece | 70905.28 | 0.49 | 26902.83 | 0.47 | 0.96 | *** | 5081.10 | 0.41 | 0.83 | *** |
| Singapore | 69488.21 | 0.48 | 26688.37 | 0.47 | 0.98 | *** | 7422.92 | 0.60 | 1.24 | *** |
| Egypt | 67862.86 | 0.47 | 31367.23 | 0.55 | 1.17 | *** | 4228.88 | 0.34 | 0.72 | *** |
| New Zealand | 67260.30 | 0.47 | 25411.26 | 0.45 | 0.96 | *** | 4890.37 | 0.39 | 0.84 | *** |
| Czechia | 60224.67 | 0.42 | 23107.18 | 0.41 | 0.97 | *** | 4636.70 | 0.37 | 0.89 | *** |
| Hungary | 37556.90 | 0.26 | 14811.82 | 0.26 | 1.00 | | 2731.37 | 0.22 | 0.84 | *** |
| *Total* | 13591963.00 | 94.14 | 5346430.89 | 94.06 | – | – | 1189790.82 | 95.75 | – | – |

* $p < 0.05$, ** $p < 0.01$, *** $p < 0.001$

Table S6: Number of papers in the 2010s by field.

| Field | All papers Count | All papers with affiliation | Novel papers Count | Novel papers with affiliation | Atypical papers Count | Atypical papers with affiliation |
|---|---|---|---|---|---|---|
| Medicine | 3596403 | 3499017.22 | 1537898 | 1497174.81 | 219207 | 212993.12 |
| Biology | 2196548 | 2153618.47 | 961015 | 942705.37 | 188796 | 185241.36 |
| Materials science | 1836415 | 1809776.34 | 736494 | 726097.91 | 253508 | 250682.45 |
| Chemistry | 1832936 | 1804571.95 | 946402 | 931859.16 | 269584 | 265371.85 |
| Psychology | 861179 | 842808.66 | 280722 | 274922.57 | 40224 | 39484.62 |
| Computer science | 830086 | 816334.41 | 336563 | 331381.15 | 56701 | 56014.12 |
| Mathematics | 676880 | 663770.06 | 183004 | 179437.56 | 37675 | 37048.54 |
| Physics | 602402 | 590313.29 | 149521 | 146554.56 | 67737 | 66417.86 |
| Engineering | 456850 | 446923.34 | 146334 | 143327.07 | 25609 | 25216.33 |
| Environmental science | 373973 | 367538.89 | 153506 | 150912.41 | 49057 | 48447.85 |
| Geology | 301295 | 296190.67 | 69722 | 68513.54 | 27349 | 26969.50 |
| Economics | 284298 | 277692.38 | 60566 | 59250.26 | 9136 | 8957.56 |
| Sociology | 261490 | 256725.27 | 54805 | 53683.33 | 2092 | 2050.36 |
| Business | 222067 | 216196.01 | 63028 | 61580.46 | 6353 | 6215.96 |
| Geography | 164022 | 159988.53 | 64357 | 62894.33 | 7681 | 7513.09 |
| Political science | 140818 | 137573.74 | 32623 | 31826.80 | 1954 | 1906.25 |
| Philosophy | 43312 | 42540.52 | 9828 | 9630.09 | 1031 | 1011.14 |
| History | 28121 | 27702.31 | 5775 | 5661.69 | 400 | 391.95 |
| Art | 21616 | 21057.59 | 5038 | 4887.68 | 506 | 489.90 |

Table S7: Statistics about the production of Medicine papers in the 2010s for 38 countries/regions.

| Country/region | All papers Count | All papers % | Novel papers Count | Novel papers % | $r_N$ | $p$-val | Atypical papers Count | Atypical papers % | $r_A$ | $p$-val |
|---|---|---|---|---|---|---|---|---|---|---|
| US | 1014773.28 | 29.00 | 435541.54 | 29.09 | 1.003 | *** | 73211.79 | 34.37 | 1.185 | *** |
| UK | 237069.20 | 6.78 | 98296.19 | 6.57 | 0.969 | *** | 14832.90 | 6.96 | 1.028 | *** |
| China | 209529.26 | 5.99 | 109504.22 | 7.31 | 1.221 | *** | 11261.57 | 5.29 | 0.883 | *** |
| Japan | 187271.62 | 5.35 | 70833.80 | 4.73 | 0.884 | *** | 12790.92 | 6.01 | 1.122 | *** |
| Germany | 131315.81 | 3.75 | 53605.71 | 3.58 | 0.954 | *** | 9496.41 | 4.46 | 1.188 | *** |
| Italy | 129025.59 | 3.69 | 48032.90 | 3.21 | 0.870 | *** | 7608.70 | 3.57 | 0.969 | ** |
| Korea | 128598.28 | 3.68 | 51900.12 | 3.47 | 0.943 | *** | 7156.55 | 3.36 | 0.914 | *** |
| Australia | 120333.15 | 3.44 | 51260.61 | 3.42 | 0.996 | | 6122.06 | 2.87 | 0.836 | *** |
| Canada | 120200.04 | 3.44 | 52091.81 | 3.48 | 1.013 | *** | 7407.82 | 3.48 | 1.012 | |
| France | 109052.86 | 3.12 | 39492.50 | 2.64 | 0.846 | *** | 7035.22 | 3.30 | 1.060 | *** |
| Spain | 103412.21 | 2.96 | 35340.01 | 2.36 | 0.799 | *** | 5176.49 | 2.43 | 0.822 | *** |
| Brazil | 92687.38 | 2.65 | 45298.45 | 3.03 | 1.142 | *** | 4213.63 | 1.98 | 0.747 | *** |
| India | 88242.97 | 2.52 | 35598.15 | 2.38 | 0.943 | *** | 3227.74 | 1.52 | 0.601 | *** |
| Netherlands | 76986.24 | 2.20 | 33747.22 | 2.25 | 1.024 | *** | 5801.38 | 2.72 | 1.238 | *** |
| Turkey | 59797.01 | 1.71 | 25325.63 | 1.69 | 0.990 | * | 2643.09 | 1.24 | 0.726 | *** |
| Iran | 58188.48 | 1.66 | 30812.22 | 2.06 | 1.238 | *** | 1697.99 | 0.80 | 0.479 | *** |
| Sweden | 42756.62 | 1.22 | 19962.88 | 1.33 | 1.091 | *** | 2813.08 | 1.32 | 1.081 | *** |
| Taiwan | 41575.37 | 1.19 | 20728.69 | 1.38 | 1.165 | *** | 2372.43 | 1.11 | 0.937 | *** |
| Switzerland | 34883.77 | 1.00 | 14822.53 | 0.99 | 0.993 | | 2808.33 | 1.32 | 1.323 | *** |
| Denmark | 32702.63 | 0.93 | 15133.96 | 1.01 | 1.082 | *** | 2130.67 | 1.00 | 1.070 | *** |
| Belgium | 29043.84 | 0.83 | 11633.53 | 0.78 | 0.936 | *** | 2014.60 | 0.95 | 1.140 | *** |
| Poland | 23665.34 | 0.68 | 11285.75 | 0.75 | 1.115 | *** | 1002.48 | 0.47 | 0.696 | *** |
| Israel | 21318.70 | 0.61 | 9153.10 | 0.61 | 1.003 | | 1220.11 | 0.57 | 0.940 | * |
| Greece | 21166.95 | 0.60 | 8396.13 | 0.56 | 0.927 | *** | 1034.52 | 0.49 | 0.803 | *** |
| Egypt | 20411.46 | 0.58 | 8821.89 | 0.59 | 1.010 | | 893.43 | 0.42 | 0.719 | *** |
| Norway | 20355.69 | 0.58 | 9108.81 | 0.61 | 1.046 | *** | 1142.44 | 0.54 | 0.922 | ** |
| South Africa | 19008.83 | 0.54 | 8922.07 | 0.60 | 1.097 | *** | 855.53 | 0.40 | 0.739 | *** |
| Austria | 18981.32 | 0.54 | 7827.43 | 0.52 | 0.964 | *** | 1459.26 | 0.69 | 1.263 | *** |
| Mexico | 18453.11 | 0.53 | 8214.25 | 0.55 | 1.040 | *** | 748.23 | 0.35 | 0.666 | *** |
| Finland | 16632.23 | 0.48 | 7648.79 | 0.51 | 1.075 | *** | 1104.05 | 0.52 | 1.090 | ** |
| Portugal | 16323.92 | 0.47 | 6543.37 | 0.44 | 0.937 | *** | 778.76 | 0.37 | 0.784 | *** |
| Hong Kong | 14240.81 | 0.41 | 6281.19 | 0.42 | 1.031 | *** | 848.74 | 0.40 | 0.979 | |
| New Zealand | 13899.19 | 0.40 | 6152.02 | 0.41 | 1.034 | *** | 734.33 | 0.34 | 0.868 | *** |
| Singapore | 11517.31 | 0.33 | 4859.81 | 0.32 | 0.986 | | 756.73 | 0.36 | 1.079 | * |
| Malaysia | 10596.74 | 0.30 | 5490.51 | 0.37 | 1.211 | *** | 397.10 | 0.19 | 0.616 | *** |
| Russia | 10350.18 | 0.30 | 4409.43 | 0.29 | 0.996 | | 391.61 | 0.18 | 0.622 | *** |
| Hungary | 6948.05 | 0.20 | 3111.36 | 0.21 | 1.047 | *** | 358.46 | 0.17 | 0.848 | *** |
| Czechia | 6903.65 | 0.20 | 2780.37 | 0.19 | 0.941 | *** | 386.79 | 0.18 | 0.920 | * |
| *Total* | 3318219.12 | 94.83 | 1417968.96 | 94.71 | – | – | 205935.93 | 96.69 | – | – |

* $p < 0.05$, ** $p < 0.01$, *** $p < 0.001$

Table S8: Statistics about the production of Biology papers in the 2010s for 38 countries/regions.

| | All papers | | Novel papers | | | | Atypical papers | | | |
|---|---|---|---|---|---|---|---|---|---|---|
| Country/region | Count | % | Count | % | $r_N$ | $p$-val | Count | % | $r_A$ | $p$-val |
| US | 584164.64 | 27.12 | 237632.18 | 25.21 | 0.929 | *** | 61714.02 | 33.32 | 1.228 | *** |
| China | 244354.68 | 11.35 | 125375.72 | 13.30 | 1.172 | *** | 18514.15 | 9.99 | 0.881 | *** |
| Japan | 106187.32 | 4.93 | 41844.79 | 4.44 | 0.900 | *** | 9149.28 | 4.94 | 1.002 | |
| UK | 105019.87 | 4.88 | 43785.70 | 4.64 | 0.952 | *** | 10519.16 | 5.68 | 1.165 | *** |
| Germany | 103984.16 | 4.83 | 42084.83 | 4.46 | 0.925 | *** | 9602.68 | 5.18 | 1.074 | *** |
| Brazil | 81356.56 | 3.78 | 36511.75 | 3.87 | 1.025 | *** | 3954.71 | 2.13 | 0.565 | *** |
| France | 69757.49 | 3.24 | 27540.57 | 2.92 | 0.902 | *** | 6576.12 | 3.55 | 1.096 | *** |
| Canada | 67634.31 | 3.14 | 27334.79 | 2.90 | 0.923 | *** | 6377.58 | 3.44 | 1.096 | *** |
| India | 63844.79 | 2.96 | 34335.91 | 3.64 | 1.229 | *** | 3625.74 | 1.96 | 0.660 | *** |
| Australia | 60919.24 | 2.83 | 24627.22 | 2.61 | 0.924 | *** | 5312.16 | 2.87 | 1.014 | |
| Italy | 59170.94 | 2.75 | 28317.76 | 3.00 | 1.093 | *** | 4362.46 | 2.36 | 0.857 | *** |
| Spain | 57933.53 | 2.69 | 23025.56 | 2.44 | 0.908 | *** | 4887.16 | 2.64 | 0.981 | |
| Korea | 53851.77 | 2.50 | 27561.97 | 2.92 | 1.169 | *** | 4135.67 | 2.23 | 0.893 | *** |
| Netherlands | 30543.89 | 1.42 | 13659.89 | 1.45 | 1.022 | *** | 3235.42 | 1.75 | 1.232 | *** |
| Iran | 23873.75 | 1.11 | 12174.13 | 1.29 | 1.165 | *** | 1118.61 | 0.60 | 0.545 | *** |
| Russia | 23342.84 | 1.08 | 8488.13 | 0.90 | 0.831 | *** | 1010.96 | 0.55 | 0.504 | *** |
| Switzerland | 23174.66 | 1.08 | 8827.20 | 0.94 | 0.870 | *** | 2334.13 | 1.26 | 1.171 | *** |
| Sweden | 22610.40 | 1.05 | 9328.36 | 0.99 | 0.943 | *** | 2128.26 | 1.15 | 1.094 | *** |
| Poland | 22191.12 | 1.03 | 9997.67 | 1.06 | 1.029 | *** | 1083.46 | 0.58 | 0.568 | *** |
| Mexico | 20717.00 | 0.96 | 8901.80 | 0.94 | 0.982 | ** | 1295.13 | 0.70 | 0.727 | *** |
| Belgium | 19880.37 | 0.92 | 8610.64 | 0.91 | 0.989 | | 1765.97 | 0.95 | 1.033 | |
| Taiwan | 19777.20 | 0.92 | 10475.92 | 1.11 | 1.210 | *** | 1684.82 | 0.91 | 0.990 | |
| Denmark | 15345.73 | 0.71 | 7033.79 | 0.75 | 1.047 | *** | 1609.28 | 0.87 | 1.219 | *** |
| South Africa | 14801.28 | 0.69 | 6108.25 | 0.65 | 0.943 | *** | 981.92 | 0.53 | 0.771 | *** |
| Israel | 13666.01 | 0.63 | 5410.84 | 0.57 | 0.905 | *** | 1232.94 | 0.67 | 1.049 | * |
| Portugal | 13255.83 | 0.62 | 6470.67 | 0.69 | 1.115 | *** | 1040.76 | 0.56 | 0.913 | *** |
| Austria | 12368.99 | 0.57 | 5219.10 | 0.55 | 0.964 | *** | 1039.97 | 0.56 | 0.978 | |
| New Zealand | 11979.29 | 0.56 | 5054.90 | 0.54 | 0.964 | *** | 990.53 | 0.53 | 0.961 | |
| Turkey | 11597.39 | 0.54 | 5587.07 | 0.59 | 1.101 | *** | 577.66 | 0.31 | 0.579 | *** |
| Norway | 10825.47 | 0.50 | 4869.38 | 0.52 | 1.028 | ** | 972.03 | 0.52 | 1.044 | |
| Czechia | 10539.30 | 0.49 | 4103.21 | 0.44 | 0.889 | *** | 638.55 | 0.34 | 0.704 | *** |
| Finland | 10476.75 | 0.49 | 4559.31 | 0.48 | 0.994 | | 980.00 | 0.53 | 1.088 | ** |
| Singapore | 8277.22 | 0.38 | 3594.05 | 0.38 | 0.992 | | 847.78 | 0.46 | 1.191 | *** |
| Malaysia | 7841.06 | 0.36 | 4717.48 | 0.50 | 1.374 | *** | 489.23 | 0.26 | 0.725 | *** |
| Egypt | 7515.24 | 0.35 | 4645.78 | 0.49 | 1.412 | *** | 306.33 | 0.17 | 0.474 | *** |
| Greece | 7155.42 | 0.33 | 3245.16 | 0.34 | 1.036 | ** | 542.57 | 0.29 | 0.882 | ** |
| Hungary | 6769.84 | 0.31 | 2694.33 | 0.29 | 0.909 | *** | 394.66 | 0.21 | 0.678 | *** |
| Hong Kong | 6380.97 | 0.30 | 3246.07 | 0.34 | 1.162 | *** | 656.95 | 0.35 | 1.197 | *** |
| *Total* | 2033086.30 | 94.40 | 887001.88 | 94.09 | – | – | 177688.79 | 95.92 | – | – |

* $p < 0.05$, ** $p < 0.01$, *** $p < 0.001$

Table S9: Statistics about the production of Materials Science papers in the 2010s for 38 countries/regions.

| | All papers | | Novel papers | | | | Atypical papers | | | |
|---|---|---|---|---|---|---|---|---|---|---|
| Country/region | Count | % | Count | % | $r_N$ | $p$-val | Count | % | $r_A$ | $p$-val |
| China | 462187.04 | 25.54 | 159844.51 | 22.01 | 0.862 | *** | 71606.59 | 28.56 | 1.119 | *** |
| US | 261441.49 | 14.45 | 120695.22 | 16.62 | 1.151 | *** | 43548.44 | 17.37 | 1.203 | *** |
| India | 108678.28 | 6.01 | 42869.31 | 5.90 | 0.983 | *** | 12553.91 | 5.01 | 0.834 | *** |
| Japan | 94244.40 | 5.21 | 34407.76 | 4.74 | 0.910 | *** | 12004.90 | 4.79 | 0.920 | *** |
| Korea | 88239.32 | 4.88 | 33543.94 | 4.62 | 0.948 | *** | 13013.63 | 5.19 | 1.065 | *** |
| Germany | 72931.65 | 4.03 | 30252.44 | 4.17 | 1.034 | *** | 9918.52 | 3.96 | 0.982 | * |
| Russia | 57816.79 | 3.19 | 19723.69 | 2.72 | 0.850 | *** | 3522.81 | 1.41 | 0.440 | *** |
| Iran | 54376.10 | 3.00 | 22734.44 | 3.13 | 1.042 | *** | 6382.44 | 2.55 | 0.847 | *** |
| UK | 51621.45 | 2.85 | 23841.52 | 3.28 | 1.151 | *** | 7294.36 | 2.91 | 1.020 | * |
| France | 47788.53 | 2.64 | 20852.95 | 2.87 | 1.088 | *** | 6740.16 | 2.69 | 1.018 | |
| Taiwan | 36062.95 | 1.99 | 13303.88 | 1.83 | 0.919 | *** | 5056.51 | 2.02 | 1.012 | |
| Italy | 33434.41 | 1.85 | 15445.56 | 2.13 | 1.151 | *** | 4365.30 | 1.74 | 0.943 | *** |
| Canada | 29073.28 | 1.61 | 13331.51 | 1.84 | 1.143 | *** | 4320.34 | 1.72 | 1.073 | *** |
| Spain | 28736.53 | 1.59 | 12274.71 | 1.69 | 1.065 | *** | 4240.53 | 1.69 | 1.065 | *** |
| Australia | 27930.46 | 1.54 | 12276.90 | 1.69 | 1.096 | *** | 4104.38 | 1.64 | 1.061 | *** |
| Poland | 26971.71 | 1.49 | 10006.17 | 1.38 | 0.925 | *** | 2231.93 | 0.89 | 0.597 | *** |
| Brazil | 26926.03 | 1.49 | 11657.53 | 1.61 | 1.079 | *** | 3123.86 | 1.25 | 0.838 | *** |
| Turkey | 22971.04 | 1.27 | 8544.88 | 1.18 | 0.927 | *** | 2399.37 | 0.96 | 0.754 | *** |
| Malaysia | 20712.67 | 1.14 | 8977.71 | 1.24 | 1.080 | *** | 1959.25 | 0.78 | 0.683 | *** |
| Singapore | 15237.23 | 0.84 | 5836.24 | 0.80 | 0.955 | *** | 2385.25 | 0.95 | 1.130 | *** |
| Switzerland | 12122.49 | 0.67 | 5832.57 | 0.80 | 1.199 | *** | 1878.55 | 0.75 | 1.119 | *** |
| Sweden | 11451.28 | 0.63 | 4908.93 | 0.68 | 1.068 | *** | 1639.82 | 0.65 | 1.034 | |
| Netherlands | 11234.87 | 0.62 | 5562.78 | 0.77 | 1.234 | *** | 1858.22 | 0.74 | 1.194 | *** |
| Mexico | 10590.89 | 0.59 | 5055.26 | 0.70 | 1.190 | *** | 1214.17 | 0.48 | 0.828 | *** |
| Czechia | 10583.84 | 0.58 | 4252.90 | 0.59 | 1.002 | | 1040.57 | 0.42 | 0.710 | *** |
| Hong Kong | 9870.35 | 0.55 | 3899.64 | 0.54 | 0.985 | | 1754.87 | 0.70 | 1.284 | *** |
| Egypt | 9654.12 | 0.53 | 4363.39 | 0.60 | 1.127 | *** | 902.48 | 0.36 | 0.675 | *** |
| Belgium | 9180.81 | 0.51 | 3819.25 | 0.53 | 1.037 | ** | 1266.82 | 0.51 | 0.996 | |
| Portugal | 8880.11 | 0.49 | 3981.51 | 0.55 | 1.118 | *** | 977.07 | 0.39 | 0.794 | *** |
| Austria | 7233.08 | 0.40 | 3118.62 | 0.43 | 1.075 | *** | 942.34 | 0.38 | 0.941 | * |
| Finland | 6038.21 | 0.33 | 2879.74 | 0.40 | 1.189 | *** | 866.21 | 0.35 | 1.036 | |
| Israel | 5873.36 | 0.32 | 2962.18 | 0.41 | 1.257 | *** | 942.33 | 0.38 | 1.158 | *** |
| Greece | 5532.84 | 0.31 | 2408.54 | 0.33 | 1.085 | *** | 748.12 | 0.30 | 0.976 | |
| New Zealand | 5427.98 | 0.30 | 2102.67 | 0.29 | 0.966 | * | 761.62 | 0.30 | 1.013 | |
| South Africa | 5157.63 | 0.28 | 2285.94 | 0.31 | 1.105 | *** | 611.97 | 0.24 | 0.857 | *** |
| Denmark | 4722.10 | 0.26 | 2255.20 | 0.31 | 1.190 | *** | 776.70 | 0.31 | 1.187 | *** |
| Norway | 3618.50 | 0.20 | 1554.87 | 0.21 | 1.071 | *** | 499.60 | 0.20 | 0.997 | |
| Hungary | 3306.39 | 0.18 | 1415.79 | 0.19 | 1.067 | *** | 363.25 | 0.14 | 0.793 | *** |
| *Total* | 1707860.20 | 94.37 | 683080.63 | 94.08 | – | – | 239817.20 | 95.67 | – | – |

* $p < 0.05$, ** $p < 0.01$, *** $p < 0.001$

Table S10: Statistics about the production of Chemistry papers in the 2010s for 38 countries/regions.

| Country/region | All papers Count | % | Novel papers Count | % | $r_N$ | $p$-val | Atypical papers Count | % | $r_A$ | $p$-val |
|---|---|---|---|---|---|---|---|---|---|---|
| China | 351993.74 | 19.51 | 175023.14 | 18.78 | 0.963 | *** | 58528.59 | 22.06 | 1.131 | *** |
| US | 289137.03 | 16.02 | 150846.58 | 16.19 | 1.010 | *** | 50442.59 | 19.01 | 1.186 | *** |
| India | 112952.30 | 6.26 | 62173.45 | 6.67 | 1.066 | *** | 15760.73 | 5.94 | 0.949 | *** |
| Japan | 96539.57 | 5.35 | 45473.31 | 4.88 | 0.912 | *** | 12786.36 | 4.82 | 0.901 | *** |
| Germany | 85599.67 | 4.74 | 40930.33 | 4.39 | 0.926 | *** | 13193.95 | 4.97 | 1.048 | *** |
| Korea | 57190.75 | 3.17 | 33203.79 | 3.56 | 1.124 | *** | 7429.37 | 2.80 | 0.883 | *** |
| UK | 56142.64 | 3.11 | 28670.60 | 3.08 | 0.989 | ** | 8941.07 | 3.37 | 1.083 | *** |
| Russia | 53512.10 | 2.97 | 21246.09 | 2.28 | 0.769 | *** | 4213.84 | 1.59 | 0.535 | *** |
| France | 50511.11 | 2.80 | 24948.07 | 2.68 | 0.956 | *** | 8048.34 | 3.03 | 1.084 | *** |
| Spain | 47771.18 | 2.65 | 22052.41 | 2.37 | 0.894 | *** | 7345.99 | 2.77 | 1.046 | *** |
| Iran | 47459.54 | 2.63 | 24319.97 | 2.61 | 0.992 | * | 6356.14 | 2.40 | 0.911 | *** |
| Brazil | 46467.14 | 2.57 | 27800.90 | 2.98 | 1.159 | *** | 4672.97 | 1.76 | 0.684 | *** |
| Italy | 43128.71 | 2.39 | 24575.52 | 2.64 | 1.103 | *** | 5739.54 | 2.16 | 0.905 | *** |
| Canada | 36840.92 | 2.04 | 18795.64 | 2.02 | 0.988 | ** | 5644.84 | 2.13 | 1.042 | *** |
| Poland | 31353.27 | 1.74 | 16894.01 | 1.81 | 1.043 | *** | 3271.95 | 1.23 | 0.710 | *** |
| Australia | 28031.27 | 1.55 | 15135.39 | 1.62 | 1.046 | *** | 4476.19 | 1.69 | 1.086 | *** |
| Turkey | 24090.25 | 1.33 | 12672.26 | 1.36 | 1.019 | ** | 2736.97 | 1.03 | 0.773 | *** |
| Taiwan | 21911.76 | 1.21 | 11686.58 | 1.25 | 1.033 | *** | 3195.25 | 1.20 | 0.992 | |
| Netherlands | 19435.51 | 1.08 | 10197.28 | 1.09 | 1.016 | * | 3297.26 | 1.24 | 1.154 | *** |
| Switzerland | 14705.02 | 0.81 | 7492.51 | 0.80 | 0.987 | * | 2580.40 | 0.97 | 1.193 | *** |
| Egypt | 14605.27 | 0.81 | 9090.15 | 0.98 | 1.205 | *** | 1325.57 | 0.50 | 0.617 | *** |
| Belgium | 14325.76 | 0.79 | 6995.26 | 0.75 | 0.946 | *** | 2122.59 | 0.80 | 1.008 | |
| Mexico | 14263.57 | 0.79 | 7671.64 | 0.82 | 1.042 | *** | 1738.38 | 0.66 | 0.829 | *** |
| Malaysia | 13088.40 | 0.73 | 7106.92 | 0.76 | 1.052 | *** | 1289.24 | 0.49 | 0.670 | *** |
| Sweden | 13004.68 | 0.72 | 6957.85 | 0.75 | 1.036 | *** | 2124.58 | 0.80 | 1.111 | *** |
| Portugal | 12927.41 | 0.72 | 7735.12 | 0.83 | 1.159 | *** | 1748.67 | 0.66 | 0.920 | *** |
| Czechia | 11396.55 | 0.63 | 6100.06 | 0.65 | 1.037 | *** | 1471.83 | 0.55 | 0.878 | *** |
| Denmark | 9553.18 | 0.53 | 5268.57 | 0.57 | 1.068 | *** | 1591.01 | 0.60 | 1.133 | *** |
| Austria | 8999.97 | 0.50 | 4968.36 | 0.53 | 1.069 | *** | 1264.05 | 0.48 | 0.955 | * |
| South Africa | 8390.19 | 0.46 | 4512.44 | 0.48 | 1.042 | *** | 969.71 | 0.37 | 0.786 | *** |
| Singapore | 8254.80 | 0.46 | 4123.44 | 0.44 | 0.967 | ** | 1487.67 | 0.56 | 1.226 | *** |
| Israel | 7118.21 | 0.39 | 3902.80 | 0.42 | 1.062 | *** | 1169.53 | 0.44 | 1.117 | *** |
| Finland | 7076.07 | 0.39 | 3780.11 | 0.41 | 1.035 | ** | 1159.21 | 0.44 | 1.114 | *** |
| Greece | 6783.28 | 0.38 | 3433.72 | 0.37 | 0.980 | * | 957.09 | 0.36 | 0.959 | |
| Hungary | 6740.08 | 0.37 | 3393.10 | 0.36 | 0.975 | * | 811.79 | 0.31 | 0.819 | *** |
| New Zealand | 6532.83 | 0.36 | 3310.54 | 0.36 | 0.981 | | 1001.50 | 0.38 | 1.042 | |
| Hong Kong | 5990.87 | 0.33 | 3072.35 | 0.33 | 0.993 | | 1028.90 | 0.39 | 1.168 | *** |
| Norway | 4994.41 | 0.28 | 2640.38 | 0.28 | 1.024 | * | 687.14 | 0.26 | 0.936 | * |
| *Total* | 1688819.01 | 93.59 | 868200.65 | 93.17 | – | – | 252610.79 | 95.19 | – | – |

Table S11: Statistics about the production of Psychology papers in the 2010s for 38 countries/regions.

| Country/region | All papers Count | % | Novel papers Count | % | $r_N$ | $p$-val | Atypical papers Count | % | $r_A$ | $p$-val |
|---|---|---|---|---|---|---|---|---|---|---|
| US | 321579.87 | 38.16 | 100057.27 | 36.39 | 0.954 | *** | 16110.88 | 40.80 | 1.069 | *** |
| UK | 75382.40 | 8.94 | 26368.98 | 9.59 | 1.072 | *** | 3555.53 | 9.00 | 1.007 | |
| Canada | 44418.37 | 5.27 | 14189.37 | 5.16 | 0.979 | *** | 2061.04 | 5.22 | 0.990 | |
| Australia | 43787.53 | 5.20 | 14429.46 | 5.25 | 1.010 | | 1477.00 | 3.74 | 0.720 | *** |
| Germany | 38189.83 | 4.53 | 12452.56 | 4.53 | 1.000 | | 2544.20 | 6.44 | 1.422 | *** |
| Netherlands | 26424.83 | 3.14 | 9493.92 | 3.45 | 1.101 | *** | 1522.02 | 3.85 | 1.229 | *** |
| Spain | 20061.05 | 2.38 | 5796.66 | 2.11 | 0.886 | *** | 648.05 | 1.64 | 0.690 | *** |
| Italy | 19166.94 | 2.27 | 6518.20 | 2.37 | 1.043 | *** | 1048.06 | 2.65 | 1.167 | *** |
| China | 18055.05 | 2.14 | 6887.74 | 2.51 | 1.169 | *** | 1444.90 | 3.66 | 1.708 | *** |
| Brazil | 16245.68 | 1.93 | 6496.81 | 2.36 | 1.226 | *** | 561.17 | 1.42 | 0.737 | *** |
| France | 15783.96 | 1.87 | 5295.21 | 1.93 | 1.028 | ** | 926.34 | 2.35 | 1.253 | *** |
| Japan | 14264.70 | 1.69 | 5352.32 | 1.95 | 1.150 | *** | 1114.87 | 2.82 | 1.668 | *** |
| Korea | 11495.85 | 1.36 | 3966.82 | 1.44 | 1.058 | *** | 473.49 | 1.20 | 0.879 | ** |
| Sweden | 11297.34 | 1.34 | 4302.44 | 1.56 | 1.168 | *** | 475.57 | 1.20 | 0.899 | ** |
| Israel | 10459.64 | 1.24 | 3096.37 | 1.13 | 0.908 | *** | 431.11 | 1.09 | 0.880 | ** |
| Belgium | 9708.44 | 1.15 | 2810.16 | 1.02 | 0.887 | *** | 452.08 | 1.14 | 0.994 | |
| Iran | 9552.33 | 1.13 | 3268.10 | 1.19 | 1.049 | *** | 194.03 | 0.49 | 0.434 | *** |
| Switzerland | 8947.39 | 1.06 | 3261.41 | 1.19 | 1.117 | *** | 611.65 | 1.55 | 1.459 | *** |
| Turkey | 8845.98 | 1.05 | 2018.51 | 0.73 | 0.700 | *** | 162.28 | 0.41 | 0.392 | *** |
| Taiwan | 8188.10 | 0.97 | 2688.54 | 0.98 | 1.007 | | 325.02 | 0.82 | 0.847 | *** |
| Norway | 7817.56 | 0.93 | 2497.78 | 0.91 | 0.979 | | 229.44 | 0.58 | 0.626 | *** |
| South Africa | 7202.87 | 0.85 | 2396.17 | 0.87 | 1.020 | | 101.67 | 0.26 | 0.301 | *** |
| Finland | 6584.34 | 0.78 | 2159.58 | 0.79 | 1.005 | | 266.50 | 0.67 | 0.864 | ** |
| Hong Kong | 6491.56 | 0.77 | 1768.14 | 0.64 | 0.835 | *** | 202.07 | 0.51 | 0.664 | *** |
| New Zealand | 6169.21 | 0.73 | 1954.08 | 0.71 | 0.971 | | 177.43 | 0.45 | 0.614 | *** |
| India | 5709.71 | 0.68 | 1929.98 | 0.70 | 1.036 | * | 192.30 | 0.49 | 0.719 | *** |
| Denmark | 5316.04 | 0.63 | 2071.78 | 0.75 | 1.195 | *** | 257.36 | 0.65 | 1.033 | |
| Portugal | 5192.98 | 0.62 | 1518.11 | 0.55 | 0.896 | *** | 147.43 | 0.37 | 0.606 | *** |
| Poland | 4547.11 | 0.54 | 1562.15 | 0.57 | 1.053 | ** | 143.89 | 0.36 | 0.675 | *** |
| Malaysia | 4197.09 | 0.50 | 1295.41 | 0.47 | 0.946 | ** | 60.70 | 0.15 | 0.309 | *** |
| Austria | 3702.05 | 0.44 | 1424.41 | 0.52 | 1.180 | *** | 221.63 | 0.56 | 1.278 | *** |
| Singapore | 2974.96 | 0.35 | 957.23 | 0.35 | 0.986 | | 131.48 | 0.33 | 0.943 | |
| Greece | 2843.45 | 0.34 | 825.15 | 0.30 | 0.890 | *** | 74.43 | 0.19 | 0.559 | *** |
| Mexico | 2800.46 | 0.33 | 991.71 | 0.36 | 1.086 | *** | 93.47 | 0.24 | 0.712 | *** |
| Russia | 2689.21 | 0.32 | 840.27 | 0.31 | 0.958 | | 101.15 | 0.26 | 0.803 | * |
| Hungary | 1802.52 | 0.21 | 654.87 | 0.24 | 1.114 | *** | 94.45 | 0.24 | 1.118 | |
| Czechia | 1477.26 | 0.18 | 542.85 | 0.20 | 1.127 | *** | 48.76 | 0.12 | 0.704 | ** |
| Egypt | 574.35 | 0.07 | 203.23 | 0.07 | 1.085 | | 13.13 | 0.03 | 0.488 | ** |
| *Total* | 809948.02 | 96.10 | 264343.77 | 96.15 | – | – | 38696.56 | 98.00 | – | – |

* $p < 0.05$, ** $p < 0.01$, *** $p < 0.001$

Table S12: Statistics about the production of Computer Science papers in the 2010s for 38 countries/regions.

| Country/region | All papers Count | All papers % | Novel papers Count | Novel papers % | $r_N$ | $p$-val | Atypical papers Count | Atypical papers % | $r_A$ | $p$-val |
|---|---|---|---|---|---|---|---|---|---|---|
| US | 161710.75 | 19.81 | 74885.31 | 22.60 | 1.141 | *** | 14092.50 | 25.16 | 1.270 | *** |
| China | 151358.10 | 18.54 | 56160.74 | 16.95 | 0.914 | *** | 11127.94 | 19.87 | 1.071 | *** |
| India | 39981.78 | 4.90 | 12758.00 | 3.85 | 0.786 | *** | 1605.81 | 2.87 | 0.585 | *** |
| UK | 39805.28 | 4.88 | 18333.57 | 5.53 | 1.135 | *** | 2970.56 | 5.30 | 1.088 | *** |
| Germany | 32097.55 | 3.93 | 13819.24 | 4.17 | 1.061 | *** | 2633.81 | 4.70 | 1.196 | *** |
| Korea | 28777.58 | 3.53 | 9468.59 | 2.86 | 0.811 | *** | 1476.46 | 2.64 | 0.748 | *** |
| Spain | 25192.17 | 3.09 | 10835.90 | 3.27 | 1.060 | *** | 1496.00 | 2.67 | 0.865 | *** |
| Italy | 24287.01 | 2.98 | 10487.05 | 3.16 | 1.064 | *** | 1660.48 | 2.96 | 0.996 | |
| Japan | 24101.81 | 2.95 | 8939.78 | 2.70 | 0.914 | *** | 1433.24 | 2.56 | 0.867 | *** |
| Canada | 24041.41 | 2.95 | 9696.99 | 2.93 | 0.994 | | 1865.51 | 3.33 | 1.131 | *** |
| France | 22662.84 | 2.78 | 9371.69 | 2.83 | 1.019 | ** | 1689.75 | 3.02 | 1.087 | *** |
| Iran | 19517.13 | 2.39 | 6628.76 | 2.00 | 0.837 | *** | 1018.80 | 1.82 | 0.761 | *** |
| Australia | 18570.94 | 2.27 | 8112.63 | 2.45 | 1.076 | *** | 1279.73 | 2.28 | 1.004 | |
| Taiwan | 17816.35 | 2.18 | 5854.58 | 1.77 | 0.810 | *** | 803.82 | 1.44 | 0.658 | *** |
| Brazil | 11975.03 | 1.47 | 5029.54 | 1.52 | 1.035 | *** | 628.30 | 1.12 | 0.765 | *** |
| Netherlands | 11653.26 | 1.43 | 5435.66 | 1.64 | 1.149 | *** | 951.28 | 1.70 | 1.190 | *** |
| Turkey | 9133.31 | 1.12 | 3415.27 | 1.03 | 0.921 | *** | 379.85 | 0.68 | 0.606 | *** |
| Poland | 9001.25 | 1.10 | 3652.17 | 1.10 | 1.000 | | 385.06 | 0.69 | 0.623 | *** |
| Switzerland | 7111.00 | 0.87 | 3594.43 | 1.08 | 1.245 | *** | 699.43 | 1.25 | 1.433 | *** |
| Singapore | 7014.24 | 0.86 | 2767.18 | 0.84 | 0.972 | * | 592.92 | 1.06 | 1.232 | *** |
| Hong Kong | 6997.12 | 0.86 | 2600.78 | 0.78 | 0.916 | *** | 567.52 | 1.01 | 1.182 | *** |
| Malaysia | 6798.25 | 0.83 | 2715.27 | 0.82 | 0.984 | | 229.18 | 0.41 | 0.491 | *** |
| Sweden | 6628.31 | 0.81 | 2559.44 | 0.77 | 0.951 | *** | 449.76 | 0.80 | 0.989 | |
| Russia | 6439.56 | 0.79 | 2490.64 | 0.75 | 0.953 | *** | 276.78 | 0.49 | 0.626 | *** |
| Belgium | 6377.05 | 0.78 | 2799.82 | 0.84 | 1.082 | *** | 516.96 | 0.92 | 1.181 | *** |
| Greece | 6285.50 | 0.77 | 2452.64 | 0.74 | 0.961 | ** | 313.08 | 0.56 | 0.726 | *** |
| Portugal | 5635.78 | 0.69 | 2477.21 | 0.75 | 1.083 | *** | 301.63 | 0.54 | 0.780 | *** |
| Mexico | 4802.60 | 0.59 | 2163.45 | 0.65 | 1.110 | *** | 249.02 | 0.44 | 0.756 | *** |
| Finland | 4617.77 | 0.57 | 1892.08 | 0.57 | 1.009 | | 281.18 | 0.50 | 0.887 | * |
| Israel | 4543.97 | 0.56 | 1933.31 | 0.58 | 1.048 | ** | 373.22 | 0.67 | 1.197 | *** |
| Austria | 4476.24 | 0.55 | 1938.48 | 0.58 | 1.067 | *** | 297.54 | 0.53 | 0.969 | |
| Denmark | 3670.44 | 0.45 | 1447.50 | 0.44 | 0.971 | | 294.22 | 0.53 | 1.168 | ** |
| Norway | 3416.93 | 0.42 | 1415.87 | 0.43 | 1.021 | | 228.12 | 0.41 | 0.973 | |
| Egypt | 3141.92 | 0.38 | 1155.35 | 0.35 | 0.906 | *** | 165.44 | 0.30 | 0.767 | *** |
| Czechia | 2872.10 | 0.35 | 1136.32 | 0.34 | 0.975 | | 139.15 | 0.25 | 0.706 | *** |
| New Zealand | 2756.25 | 0.34 | 1222.84 | 0.37 | 1.093 | *** | 162.39 | 0.29 | 0.859 | * |
| South Africa | 2449.64 | 0.30 | 991.61 | 0.30 | 0.997 | | 140.07 | 0.25 | 0.833 | * |
| Hungary | 1805.24 | 0.22 | 815.05 | 0.25 | 1.112 | *** | 130.27 | 0.23 | 1.052 | |
| *Total* | 769523.50 | 94.27 | 313454.73 | 94.59 | – | – | 53906.78 | 96.24 | – | – |

* $p < 0.05$, ** $p < 0.01$, *** $p < 0.001$

Table S13: Statistics about the production of Mathematics papers in the 2010s for 38 countries/regions.

| Country/region | All papers Count | % | Novel papers Count | % | $r_N$ | $p$-val | Atypical papers Count | % | $r_A$ | $p$-val |
|---|---|---|---|---|---|---|---|---|---|---|
| China | 120867.32 | 18.21 | 28797.03 | 16.05 | 0.881 | *** | 6869.85 | 18.54 | 1.018 | * |
| US | 115328.69 | 17.37 | 36525.34 | 20.36 | 1.172 | *** | 8240.18 | 22.24 | 1.280 | *** |
| France | 29481.00 | 4.44 | 8272.89 | 4.61 | 1.038 | *** | 1559.01 | 4.21 | 0.947 | * |
| Germany | 28113.58 | 4.24 | 7702.22 | 4.29 | 1.013 | | 1604.06 | 4.33 | 1.022 | |
| UK | 25289.23 | 3.81 | 8076.39 | 4.50 | 1.181 | *** | 1661.75 | 4.49 | 1.177 | *** |
| India | 23336.67 | 3.52 | 6168.52 | 3.44 | 0.978 | * | 1055.40 | 2.85 | 0.810 | *** |
| Italy | 21599.19 | 3.25 | 5941.82 | 3.31 | 1.018 | | 1128.32 | 3.05 | 0.936 | ** |
| Russia | 21086.05 | 3.18 | 3971.65 | 2.21 | 0.697 | *** | 362.13 | 0.98 | 0.308 | *** |
| Iran | 20315.57 | 3.06 | 5244.70 | 2.92 | 0.955 | *** | 1042.19 | 2.81 | 0.919 | ** |
| Japan | 19355.20 | 2.92 | 4353.58 | 2.43 | 0.832 | *** | 968.43 | 2.61 | 0.896 | *** |
| Spain | 19031.34 | 2.87 | 5217.85 | 2.91 | 1.014 | | 1061.83 | 2.87 | 1.000 | |
| Canada | 18251.17 | 2.75 | 5331.76 | 2.97 | 1.081 | *** | 1241.68 | 3.35 | 1.219 | *** |
| Brazil | 14440.99 | 2.18 | 4062.42 | 2.26 | 1.041 | ** | 808.36 | 2.18 | 1.003 | |
| Korea | 13725.62 | 2.07 | 3209.19 | 1.79 | 0.865 | *** | 810.67 | 2.19 | 1.058 | * |
| Australia | 11492.77 | 1.73 | 3729.30 | 2.08 | 1.200 | *** | 791.06 | 2.14 | 1.233 | *** |
| Turkey | 10768.64 | 1.62 | 2492.14 | 1.39 | 0.856 | *** | 375.54 | 1.01 | 0.625 | *** |
| Poland | 10313.93 | 1.55 | 2382.50 | 1.33 | 0.855 | *** | 358.57 | 0.97 | 0.623 | *** |
| Taiwan | 8828.87 | 1.33 | 2319.66 | 1.29 | 0.972 | | 536.16 | 1.45 | 1.088 | * |
| Netherlands | 6620.72 | 1.00 | 2369.11 | 1.32 | 1.324 | *** | 522.33 | 1.41 | 1.413 | *** |
| Israel | 6398.44 | 0.96 | 1485.96 | 0.83 | 0.859 | *** | 298.28 | 0.81 | 0.835 | *** |
| Belgium | 5405.36 | 0.81 | 1743.73 | 0.97 | 1.193 | *** | 362.71 | 0.98 | 1.202 | *** |
| Mexico | 5291.02 | 0.80 | 1722.07 | 0.96 | 1.204 | *** | 294.74 | 0.80 | 0.998 | |
| Switzerland | 5055.72 | 0.76 | 1524.48 | 0.85 | 1.115 | *** | 368.49 | 0.99 | 1.306 | *** |
| Sweden | 4947.43 | 0.75 | 1470.38 | 0.82 | 1.099 | *** | 272.63 | 0.74 | 0.987 | |
| Austria | 4691.27 | 0.71 | 1246.23 | 0.69 | 0.983 | | 194.17 | 0.52 | 0.742 | *** |
| Hong Kong | 4566.93 | 0.69 | 1259.91 | 0.70 | 1.021 | | 347.32 | 0.94 | 1.363 | *** |
| Czechia | 4372.38 | 0.66 | 1002.96 | 0.56 | 0.849 | *** | 161.00 | 0.43 | 0.660 | *** |
| Portugal | 4347.73 | 0.66 | 1199.42 | 0.67 | 1.021 | | 197.65 | 0.53 | 0.814 | ** |
| Greece | 3835.67 | 0.58 | 1182.74 | 0.66 | 1.141 | *** | 236.92 | 0.64 | 1.107 | |
| Singapore | 3309.63 | 0.50 | 877.17 | 0.49 | 0.980 | | 270.64 | 0.73 | 1.465 | *** |
| South Africa | 3274.31 | 0.49 | 944.22 | 0.53 | 1.067 | * | 155.39 | 0.42 | 0.850 | * |
| Hungary | 3232.25 | 0.49 | 794.95 | 0.44 | 0.910 | *** | 111.51 | 0.30 | 0.618 | *** |
| Finland | 2962.14 | 0.45 | 822.18 | 0.46 | 1.027 | | 181.64 | 0.49 | 1.099 | |
| Egypt | 2851.26 | 0.43 | 731.19 | 0.41 | 0.949 | * | 96.65 | 0.26 | 0.607 | *** |
| Norway | 2840.34 | 0.43 | 808.35 | 0.45 | 1.053 | * | 183.82 | 0.50 | 1.159 | * |
| Malaysia | 2570.72 | 0.39 | 922.65 | 0.51 | 1.328 | *** | 127.86 | 0.35 | 0.891 | |
| Denmark | 2409.95 | 0.36 | 817.32 | 0.46 | 1.255 | *** | 181.26 | 0.49 | 1.348 | *** |
| New Zealand | 1974.32 | 0.30 | 651.99 | 0.36 | 1.222 | *** | 123.97 | 0.33 | 1.125 | |
| *Total* | 612583.42 | 92.29 | 167375.96 | 93.28 | – | – | 35164.18 | 94.91 | – | – |

* $p < 0.05$, ** $p < 0.01$, *** $p < 0.001$

Table S14: Statistics about the production of Physics papers in the 2010s for 38 countries/regions.

| Country/region | All papers Count | % | Novel papers Count | % | $r_N$ | $p$-val | Atypical papers Count | % | $r_A$ | $p$-val |
|---|---|---|---|---|---|---|---|---|---|---|
| US | 127700.24 | 21.63 | 33838.15 | 23.09 | 1.067 | *** | 16802.06 | 25.30 | 1.169 | *** |
| China | 72306.74 | 12.25 | 17531.53 | 11.96 | 0.977 | *** | 7700.76 | 11.59 | 0.947 | *** |
| Germany | 40255.96 | 6.82 | 9232.20 | 6.30 | 0.924 | *** | 4708.47 | 7.09 | 1.040 | ** |
| Russia | 32554.22 | 5.51 | 7323.09 | 5.00 | 0.906 | *** | 2378.38 | 3.58 | 0.649 | *** |
| UK | 30330.66 | 5.14 | 7577.28 | 5.17 | 1.006 | | 3627.89 | 5.46 | 1.063 | *** |
| Japan | 29536.30 | 5.00 | 6387.65 | 4.36 | 0.871 | *** | 3048.84 | 4.59 | 0.917 | *** |
| France | 25418.83 | 4.31 | 7242.13 | 4.94 | 1.148 | *** | 3446.59 | 5.19 | 1.205 | *** |
| India | 23044.42 | 3.90 | 5050.86 | 3.45 | 0.883 | *** | 2417.17 | 3.64 | 0.932 | *** |
| Italy | 21522.18 | 3.65 | 5261.66 | 3.59 | 0.985 | | 2364.83 | 3.56 | 0.977 | |
| Spain | 14265.98 | 2.42 | 3300.69 | 2.25 | 0.932 | *** | 1552.06 | 2.34 | 0.967 | |
| Brazil | 13467.26 | 2.28 | 3593.66 | 2.45 | 1.075 | *** | 1230.00 | 1.85 | 0.812 | *** |
| Canada | 12432.10 | 2.11 | 3254.86 | 2.22 | 1.055 | *** | 1572.52 | 2.37 | 1.124 | *** |
| Korea | 11943.82 | 2.02 | 2718.09 | 1.85 | 0.917 | *** | 1140.10 | 1.72 | 0.848 | *** |
| Iran | 11727.71 | 1.99 | 2807.45 | 1.92 | 0.964 | * | 1001.21 | 1.51 | 0.759 | *** |
| Australia | 8990.74 | 1.52 | 2409.48 | 1.64 | 1.079 | *** | 1082.84 | 1.63 | 1.070 | ** |
| Switzerland | 8337.72 | 1.41 | 1900.21 | 1.30 | 0.918 | *** | 901.94 | 1.36 | 0.961 | |
| Poland | 7004.06 | 1.19 | 1685.62 | 1.15 | 0.969 | | 638.01 | 0.96 | 0.810 | *** |
| Netherlands | 6864.96 | 1.16 | 1840.75 | 1.26 | 1.080 | *** | 916.30 | 1.38 | 1.186 | *** |
| Taiwan | 5869.48 | 0.99 | 1251.86 | 0.85 | 0.859 | *** | 576.44 | 0.87 | 0.873 | *** |
| Mexico | 5155.09 | 0.87 | 1328.89 | 0.91 | 1.038 | | 543.67 | 0.82 | 0.937 | |
| Sweden | 4935.68 | 0.84 | 1387.91 | 0.95 | 1.133 | *** | 693.49 | 1.04 | 1.249 | *** |
| Israel | 4932.47 | 0.84 | 1326.95 | 0.91 | 1.084 | *** | 666.81 | 1.00 | 1.202 | *** |
| Turkey | 4891.17 | 0.83 | 1231.80 | 0.84 | 1.014 | | 375.95 | 0.57 | 0.683 | *** |
| Belgium | 4395.12 | 0.74 | 1085.91 | 0.74 | 0.995 | | 538.95 | 0.81 | 1.090 | * |
| Austria | 3389.23 | 0.57 | 878.54 | 0.60 | 1.044 | | 429.54 | 0.65 | 1.126 | ** |
| Czechia | 2980.48 | 0.50 | 720.64 | 0.49 | 0.974 | | 300.67 | 0.45 | 0.897 | * |
| Denmark | 2615.51 | 0.44 | 573.54 | 0.39 | 0.883 | *** | 287.63 | 0.43 | 0.977 | |
| Finland | 2524.95 | 0.43 | 617.29 | 0.42 | 0.985 | | 284.42 | 0.43 | 1.001 | |
| Singapore | 2470.27 | 0.42 | 728.81 | 0.50 | 1.188 | *** | 328.01 | 0.49 | 1.180 | *** |
| Greece | 2453.35 | 0.42 | 684.28 | 0.47 | 1.123 | *** | 297.87 | 0.45 | 1.079 | |
| Portugal | 2444.79 | 0.41 | 553.47 | 0.38 | 0.912 | ** | 250.72 | 0.38 | 0.911 | |
| Egypt | 2167.15 | 0.37 | 563.90 | 0.38 | 1.048 | | 187.43 | 0.28 | 0.769 | *** |
| Hong Kong | 2093.22 | 0.35 | 551.90 | 0.38 | 1.062 | | 282.20 | 0.42 | 1.198 | *** |
| South Africa | 2030.62 | 0.34 | 378.85 | 0.26 | 0.751 | *** | 165.91 | 0.25 | 0.726 | *** |
| Hungary | 1868.56 | 0.32 | 492.94 | 0.34 | 1.063 | | 220.44 | 0.33 | 1.049 | |
| Norway | 1759.45 | 0.30 | 548.91 | 0.37 | 1.257 | *** | 234.59 | 0.35 | 1.185 | ** |
| New Zealand | 1300.25 | 0.22 | 435.15 | 0.30 | 1.348 | *** | 166.46 | 0.25 | 1.138 | * |
| Malaysia | 1155.23 | 0.20 | 395.83 | 0.27 | 1.380 | *** | 91.19 | 0.14 | 0.702 | *** |
| *Total* | 559135.97 | 94.72 | 138692.69 | 94.64 | – | – | 63452.36 | 95.54 | – | – |

* $p < 0.05$, ** $p < 0.01$, *** $p < 0.001$

Table S15: Statistics about the production of Engineering papers in the 2010s for 38 countries/regions.

| | All papers | | Novel papers | | | | Atypical papers | | | |
|---|---|---|---|---|---|---|---|---|---|---|
| Country/region | Count | % | Count | % | $r_N$ | $p$-val | Count | % | $r_A$ | $p$-val |
| China | 84874.48 | 18.99 | 23683.46 | 16.52 | 0.870 | *** | 3803.47 | 15.08 | 0.794 | *** |
| US | 69263.75 | 15.50 | 26844.84 | 18.73 | 1.209 | *** | 4759.31 | 18.87 | 1.218 | *** |
| UK | 21037.21 | 4.71 | 8090.71 | 5.64 | 1.199 | *** | 1361.08 | 5.40 | 1.147 | *** |
| India | 19883.31 | 4.45 | 4884.97 | 3.41 | 0.766 | *** | 1026.74 | 4.07 | 0.915 | ** |
| Italy | 18140.15 | 4.06 | 5924.65 | 4.13 | 1.018 | * | 1138.87 | 4.52 | 1.113 | *** |
| Korea | 16613.23 | 3.72 | 4705.23 | 3.28 | 0.883 | *** | 767.88 | 3.05 | 0.819 | *** |
| Iran | 15372.12 | 3.44 | 4068.33 | 2.84 | 0.825 | *** | 843.13 | 3.34 | 0.972 | |
| Germany | 13964.18 | 3.12 | 4746.74 | 3.31 | 1.060 | *** | 793.87 | 3.15 | 1.008 | |
| Canada | 13625.32 | 3.05 | 4465.37 | 3.12 | 1.022 | * | 909.54 | 3.61 | 1.183 | *** |
| Spain | 12718.21 | 2.85 | 4322.69 | 3.02 | 1.060 | *** | 859.69 | 3.41 | 1.198 | *** |
| Australia | 12580.12 | 2.81 | 4463.57 | 3.11 | 1.106 | *** | 704.34 | 2.79 | 0.992 | |
| France | 11358.88 | 2.54 | 4022.47 | 2.81 | 1.104 | *** | 719.73 | 2.85 | 1.123 | *** |
| Japan | 10699.49 | 2.39 | 3051.71 | 2.13 | 0.889 | *** | 488.17 | 1.94 | 0.809 | *** |
| Taiwan | 10566.64 | 2.36 | 3012.85 | 2.10 | 0.889 | *** | 535.37 | 2.12 | 0.898 | ** |
| Malaysia | 7680.74 | 1.72 | 2543.97 | 1.77 | 1.033 | * | 381.48 | 1.51 | 0.880 | ** |
| Brazil | 7153.74 | 1.60 | 2240.49 | 1.56 | 0.977 | | 422.29 | 1.67 | 1.046 | |
| Turkey | 6787.70 | 1.52 | 1835.09 | 1.28 | 0.843 | *** | 357.93 | 1.42 | 0.935 | |
| Poland | 6085.30 | 1.36 | 1722.34 | 1.20 | 0.883 | *** | 223.42 | 0.89 | 0.651 | *** |
| Sweden | 5770.48 | 1.29 | 1973.57 | 1.38 | 1.066 | *** | 353.73 | 1.40 | 1.086 | |
| Netherlands | 5521.34 | 1.24 | 2224.99 | 1.55 | 1.257 | *** | 388.56 | 1.54 | 1.247 | *** |
| Portugal | 4398.62 | 0.98 | 1384.39 | 0.97 | 0.981 | | 267.33 | 1.06 | 1.077 | |
| Greece | 3871.61 | 0.87 | 1198.98 | 0.84 | 0.966 | | 261.61 | 1.04 | 1.198 | ** |
| Hong Kong | 3760.75 | 0.84 | 1169.41 | 0.82 | 0.970 | | 291.32 | 1.16 | 1.373 | *** |
| Singapore | 3493.73 | 0.78 | 1174.49 | 0.82 | 1.048 | * | 258.10 | 1.02 | 1.309 | *** |
| Norway | 3269.30 | 0.73 | 1133.17 | 0.79 | 1.081 | *** | 161.37 | 0.64 | 0.875 | * |
| Switzerland | 3242.45 | 0.73 | 1332.95 | 0.93 | 1.282 | *** | 270.46 | 1.07 | 1.478 | *** |
| Belgium | 3147.17 | 0.70 | 1162.89 | 0.81 | 1.152 | *** | 234.00 | 0.93 | 1.318 | *** |
| Mexico | 2931.10 | 0.66 | 950.66 | 0.66 | 1.011 | | 143.16 | 0.57 | 0.866 | * |
| Russia | 2777.21 | 0.62 | 678.19 | 0.47 | 0.761 | *** | 63.27 | 0.25 | 0.404 | *** |
| Denmark | 2771.64 | 0.62 | 833.83 | 0.58 | 0.938 | * | 206.97 | 0.82 | 1.324 | *** |
| Finland | 2477.41 | 0.55 | 871.94 | 0.61 | 1.097 | *** | 148.37 | 0.59 | 1.061 | |
| Egypt | 2430.73 | 0.54 | 525.52 | 0.37 | 0.674 | *** | 122.73 | 0.49 | 0.895 | |
| South Africa | 2089.83 | 0.47 | 749.35 | 0.52 | 1.118 | *** | 108.32 | 0.43 | 0.919 | |
| Austria | 2031.69 | 0.45 | 721.76 | 0.50 | 1.108 | *** | 118.57 | 0.47 | 1.034 | |
| New Zealand | 1890.11 | 0.42 | 645.64 | 0.45 | 1.065 | * | 104.83 | 0.42 | 0.983 | |
| Czechia | 1843.16 | 0.41 | 545.49 | 0.38 | 0.923 | * | 62.68 | 0.25 | 0.603 | *** |
| Israel | 1480.07 | 0.33 | 584.84 | 0.41 | 1.232 | *** | 108.18 | 0.43 | 1.295 | ** |
| Hungary | 891.17 | 0.20 | 254.60 | 0.18 | 0.891 | * | 49.84 | 0.20 | 0.991 | |
| *Total* | 418494.15 | 93.64 | 134746.14 | 94.01 | – | – | 23819.70 | 94.46 | – | – |

* $p < 0.05$, ** $p < 0.01$, *** $p < 0.001$

Table S16: Statistics about the production of Environmental Science papers in the 2010s for 38 countries/regions.

| Country/region | All papers Count | All papers % | Novel papers Count | Novel papers % | Novel papers $r_N$ | Novel papers $p$-val | Atypical papers Count | Atypical papers % | Atypical papers $r_A$ | Atypical papers $p$-val |
|---|---|---|---|---|---|---|---|---|---|---|
| US | 94381.28 | 25.68 | 38263.91 | 25.36 | 0.987 | *** | 14159.80 | 29.23 | 1.138 | *** |
| China | 46304.68 | 12.60 | 19573.45 | 12.97 | 1.029 | *** | 6733.89 | 13.90 | 1.103 | *** |
| UK | 15725.39 | 4.28 | 6672.35 | 4.42 | 1.033 | *** | 2167.02 | 4.47 | 1.045 | * |
| India | 14789.89 | 4.02 | 5926.77 | 3.93 | 0.976 | ** | 1544.52 | 3.19 | 0.792 | *** |
| Canada | 14278.19 | 3.88 | 5596.98 | 3.71 | 0.955 | *** | 1952.03 | 4.03 | 1.037 | * |
| Germany | 13824.54 | 3.76 | 5507.90 | 3.65 | 0.970 | ** | 2068.68 | 4.27 | 1.135 | *** |
| Australia | 11917.91 | 3.24 | 4974.84 | 3.30 | 1.017 | | 1526.23 | 3.15 | 0.972 | |
| Spain | 11440.46 | 3.11 | 4544.24 | 3.01 | 0.967 | ** | 1596.97 | 3.30 | 1.059 | ** |
| Japan | 10434.63 | 2.84 | 3901.74 | 2.59 | 0.911 | *** | 1146.63 | 2.37 | 0.834 | *** |
| Brazil | 9744.21 | 2.65 | 4202.11 | 2.78 | 1.050 | *** | 879.84 | 1.82 | 0.685 | *** |
| France | 9637.85 | 2.62 | 3708.37 | 2.46 | 0.937 | *** | 1390.03 | 2.87 | 1.094 | *** |
| Italy | 9608.03 | 2.61 | 4318.20 | 2.86 | 1.095 | *** | 1293.82 | 2.67 | 1.022 | |
| Korea | 6623.90 | 1.80 | 2577.44 | 1.71 | 0.948 | *** | 798.17 | 1.65 | 0.914 | ** |
| Iran | 6343.54 | 1.73 | 2457.84 | 1.63 | 0.944 | *** | 550.96 | 1.14 | 0.659 | *** |
| Netherlands | 5205.01 | 1.42 | 2405.46 | 1.59 | 1.126 | *** | 784.31 | 1.62 | 1.143 | *** |
| Russia | 5132.25 | 1.40 | 1619.77 | 1.07 | 0.769 | *** | 313.06 | 0.65 | 0.463 | *** |
| Poland | 4773.24 | 1.30 | 1790.41 | 1.19 | 0.914 | *** | 347.08 | 0.72 | 0.552 | *** |
| Sweden | 4452.36 | 1.21 | 1764.19 | 1.17 | 0.965 | * | 630.31 | 1.30 | 1.074 | * |
| Switzerland | 3772.99 | 1.03 | 1542.11 | 1.02 | 0.995 | | 605.90 | 1.25 | 1.218 | *** |
| Turkey | 3498.53 | 0.95 | 1364.15 | 0.90 | 0.950 | ** | 341.10 | 0.70 | 0.740 | *** |
| Finland | 3113.45 | 0.85 | 1199.17 | 0.79 | 0.938 | ** | 411.22 | 0.85 | 1.002 | |
| Malaysia | 2950.00 | 0.80 | 1373.38 | 0.91 | 1.134 | *** | 285.98 | 0.59 | 0.735 | *** |
| Portugal | 2896.98 | 0.79 | 1284.09 | 0.85 | 1.080 | *** | 375.12 | 0.77 | 0.982 | |
| Belgium | 2839.29 | 0.77 | 1196.99 | 0.79 | 1.027 | | 420.50 | 0.87 | 1.124 | ** |
| Norway | 2822.02 | 0.77 | 1127.96 | 0.75 | 0.973 | | 391.30 | 0.81 | 1.052 | |
| Taiwan | 2733.31 | 0.74 | 1184.13 | 0.78 | 1.055 | ** | 424.71 | 0.88 | 1.179 | *** |
| Greece | 2623.19 | 0.71 | 1040.26 | 0.69 | 0.966 | | 293.93 | 0.61 | 0.850 | ** |
| South Africa | 2620.61 | 0.71 | 1128.96 | 0.75 | 1.049 | * | 198.88 | 0.41 | 0.576 | *** |
| Denmark | 2612.56 | 0.71 | 1073.26 | 0.71 | 1.000 | | 371.39 | 0.77 | 1.078 | |
| Mexico | 2378.87 | 0.65 | 1103.09 | 0.73 | 1.129 | *** | 250.37 | 0.52 | 0.798 | *** |
| New Zealand | 2291.78 | 0.62 | 858.07 | 0.57 | 0.912 | *** | 268.12 | 0.55 | 0.888 | * |
| Austria | 1835.92 | 0.50 | 783.84 | 0.52 | 1.040 | | 240.02 | 0.50 | 0.992 | |
| Hong Kong | 1745.20 | 0.47 | 773.43 | 0.51 | 1.079 | ** | 359.64 | 0.74 | 1.563 | *** |
| Czechia | 1586.57 | 0.43 | 631.01 | 0.42 | 0.969 | | 177.79 | 0.37 | 0.850 | * |
| Israel | 1340.78 | 0.36 | 705.68 | 0.47 | 1.282 | *** | 227.77 | 0.47 | 1.289 | *** |
| Egypt | 1271.04 | 0.35 | 544.97 | 0.36 | 1.044 | | 104.16 | 0.21 | 0.622 | *** |
| Singapore | 1012.61 | 0.28 | 476.04 | 0.32 | 1.145 | *** | 185.36 | 0.38 | 1.389 | *** |
| Hungary | 752.29 | 0.20 | 317.79 | 0.21 | 1.029 | | 71.98 | 0.15 | 0.726 | ** |
| *Total* | 341315.33 | 92.87 | 139514.35 | 92.45 | – | – | 45888.60 | 94.72 | – | – |

* $p < 0.05$, ** $p < 0.01$, *** $p < 0.001$

Table S17: Statistics about the production of Geology papers in the 2010s for 38 countries/regions.

| Country/region | All papers Count | All papers % | Novel papers Count | Novel papers % | $r_N$ | $p$-val | Atypical papers Count | Atypical papers % | $r_A$ | $p$-val |
|---|---|---|---|---|---|---|---|---|---|---|
| US | 68116.65 | 23.00 | 16606.92 | 24.24 | 1.054 | *** | 7842.02 | 29.08 | 1.264 | *** |
| China | 39058.79 | 13.19 | 8380.47 | 12.23 | 0.928 | *** | 2717.81 | 10.08 | 0.764 | *** |
| UK | 16204.84 | 5.47 | 3799.63 | 5.55 | 1.014 | | 1603.79 | 5.95 | 1.087 | *** |
| Germany | 13053.79 | 4.41 | 3175.42 | 4.63 | 1.052 | *** | 1443.62 | 5.35 | 1.215 | *** |
| Russia | 12626.48 | 4.26 | 2436.89 | 3.56 | 0.834 | *** | 672.83 | 2.49 | 0.585 | *** |
| France | 12331.10 | 4.16 | 2864.50 | 4.18 | 1.004 | | 1387.39 | 5.14 | 1.236 | *** |
| Japan | 11751.64 | 3.97 | 2566.04 | 3.75 | 0.944 | *** | 1158.92 | 4.30 | 1.083 | ** |
| Canada | 11278.68 | 3.81 | 2633.70 | 3.84 | 1.009 | | 1106.50 | 4.10 | 1.077 | ** |
| Italy | 10699.59 | 3.61 | 2700.29 | 3.94 | 1.091 | *** | 1076.31 | 3.99 | 1.105 | *** |
| Australia | 10487.43 | 3.54 | 2478.09 | 3.62 | 1.022 | | 985.79 | 3.66 | 1.032 | |
| India | 9455.54 | 3.19 | 2022.42 | 2.95 | 0.925 | *** | 614.73 | 2.28 | 0.714 | *** |
| Spain | 6816.11 | 2.30 | 1612.67 | 2.35 | 1.023 | | 542.79 | 2.01 | 0.875 | *** |
| Iran | 4715.73 | 1.59 | 1069.18 | 1.56 | 0.980 | | 300.96 | 1.12 | 0.701 | *** |
| Brazil | 4398.32 | 1.48 | 977.57 | 1.43 | 0.961 | | 294.63 | 1.09 | 0.736 | *** |
| Switzerland | 4096.84 | 1.38 | 1066.47 | 1.56 | 1.125 | *** | 554.18 | 2.05 | 1.486 | *** |
| Norway | 3611.90 | 1.22 | 735.66 | 1.07 | 0.881 | *** | 336.02 | 1.25 | 1.022 | |
| Poland | 3611.69 | 1.22 | 821.10 | 1.20 | 0.983 | | 169.67 | 0.63 | 0.516 | *** |
| Netherlands | 3458.48 | 1.17 | 832.09 | 1.21 | 1.040 | | 376.60 | 1.40 | 1.196 | *** |
| Korea | 3227.37 | 1.09 | 745.60 | 1.09 | 0.999 | | 260.50 | 0.97 | 0.886 | * |
| Turkey | 3114.26 | 1.05 | 631.22 | 0.92 | 0.876 | *** | 181.48 | 0.67 | 0.640 | *** |
| New Zealand | 2743.96 | 0.93 | 519.15 | 0.76 | 0.818 | *** | 213.98 | 0.79 | 0.856 | ** |
| Taiwan | 2340.60 | 0.79 | 547.15 | 0.80 | 1.011 | | 233.15 | 0.86 | 1.094 | |
| Sweden | 2298.08 | 0.78 | 510.63 | 0.75 | 0.961 | | 199.60 | 0.74 | 0.954 | |
| Mexico | 2086.90 | 0.70 | 511.19 | 0.75 | 1.059 | | 155.78 | 0.58 | 0.820 | ** |
| South Africa | 1914.02 | 0.65 | 419.60 | 0.61 | 0.948 | | 101.16 | 0.38 | 0.580 | *** |
| Egypt | 1744.47 | 0.59 | 397.93 | 0.58 | 0.986 | | 85.72 | 0.32 | 0.540 | *** |
| Greece | 1627.13 | 0.55 | 449.71 | 0.66 | 1.195 | *** | 133.94 | 0.50 | 0.904 | |
| Belgium | 1621.88 | 0.55 | 457.80 | 0.67 | 1.220 | *** | 171.82 | 0.64 | 1.163 | * |
| Denmark | 1580.65 | 0.53 | 320.64 | 0.47 | 0.877 | ** | 154.78 | 0.57 | 1.075 | |
| Portugal | 1554.74 | 0.52 | 442.19 | 0.65 | 1.230 | *** | 142.49 | 0.53 | 1.007 | |
| Czechia | 1450.18 | 0.49 | 306.09 | 0.45 | 0.912 | * | 104.93 | 0.39 | 0.795 | ** |
| Austria | 1447.54 | 0.49 | 343.97 | 0.50 | 1.027 | | 134.01 | 0.50 | 1.017 | |
| Israel | 1239.62 | 0.42 | 396.29 | 0.58 | 1.382 | *** | 142.51 | 0.53 | 1.263 | ** |
| Hong Kong | 1221.06 | 0.41 | 240.35 | 0.35 | 0.851 | ** | 104.77 | 0.39 | 0.942 | |
| Finland | 891.08 | 0.30 | 232.74 | 0.34 | 1.129 | * | 73.85 | 0.27 | 0.910 | |
| Malaysia | 822.95 | 0.28 | 247.70 | 0.36 | 1.301 | *** | 49.38 | 0.18 | 0.659 | *** |
| Hungary | 760.91 | 0.26 | 215.33 | 0.31 | 1.223 | *** | 64.71 | 0.24 | 0.934 | |
| Singapore | 549.04 | 0.19 | 142.27 | 0.21 | 1.120 | | 53.04 | 0.20 | 1.061 | |
| *Total* | 280010.04 | 94.54 | 64856.64 | 94.66 | – | – | 25946.17 | 96.21 | – | – |

* $p < 0.05$, ** $p < 0.01$, *** $p < 0.001$

Table S18: Statistics about the production of Economics papers in the 2010s for 38 countries/regions.

| Country/region | All papers Count | All papers % | Novel papers Count | Novel papers % | $r_N$ | $p$-val | Atypical papers Count | Atypical papers % | $r_A$ | $p$-val |
|---|---|---|---|---|---|---|---|---|---|---|
| US | 74394.45 | 26.79 | 16420.90 | 27.71 | 1.034 | *** | 2634.34 | 29.41 | 1.098 | *** |
| UK | 25066.95 | 9.03 | 5459.42 | 9.21 | 1.021 | * | 655.74 | 7.32 | 0.811 | *** |
| Germany | 14697.71 | 5.29 | 3020.77 | 5.10 | 0.963 | ** | 497.74 | 5.56 | 1.050 | |
| China | 13757.74 | 4.95 | 3785.05 | 6.39 | 1.289 | *** | 855.04 | 9.55 | 1.927 | *** |
| Australia | 12203.10 | 4.39 | 2859.41 | 4.83 | 1.098 | *** | 307.57 | 3.43 | 0.781 | *** |
| Italy | 9406.31 | 3.39 | 1948.82 | 3.29 | 0.971 | | 275.48 | 3.08 | 0.908 | * |
| Canada | 9278.20 | 3.34 | 2033.96 | 3.43 | 1.027 | | 306.92 | 3.43 | 1.026 | |
| France | 8079.80 | 2.91 | 1525.20 | 2.57 | 0.885 | *** | 288.66 | 3.22 | 1.108 | * |
| Spain | 8063.23 | 2.90 | 1540.87 | 2.60 | 0.896 | *** | 245.02 | 2.74 | 0.942 | |
| Netherlands | 6546.62 | 2.36 | 1709.39 | 2.89 | 1.224 | *** | 219.31 | 2.45 | 1.039 | |
| Japan | 6227.15 | 2.24 | 1058.25 | 1.79 | 0.796 | *** | 190.47 | 2.13 | 0.948 | |
| India | 5619.64 | 2.02 | 1028.24 | 1.74 | 0.858 | *** | 132.11 | 1.47 | 0.729 | *** |
| Taiwan | 4467.55 | 1.61 | 656.49 | 1.11 | 0.689 | *** | 98.96 | 1.10 | 0.687 | *** |
| Sweden | 4284.43 | 1.54 | 1069.51 | 1.81 | 1.170 | *** | 139.23 | 1.55 | 1.007 | |
| Korea | 3961.50 | 1.43 | 656.54 | 1.11 | 0.777 | *** | 110.12 | 1.23 | 0.862 | |
| Switzerland | 3799.06 | 1.37 | 860.69 | 1.45 | 1.062 | * | 139.03 | 1.55 | 1.135 | |
| Turkey | 3576.24 | 1.29 | 583.51 | 0.98 | 0.765 | *** | 109.61 | 1.22 | 0.950 | |
| Brazil | 3417.05 | 1.23 | 716.42 | 1.21 | 0.983 | | 117.63 | 1.31 | 1.067 | |
| South Africa | 3268.20 | 1.18 | 715.86 | 1.21 | 1.027 | | 43.79 | 0.49 | 0.415 | *** |
| Belgium | 2890.85 | 1.04 | 553.63 | 0.93 | 0.898 | ** | 62.17 | 0.69 | 0.667 | *** |
| Greece | 2747.27 | 0.99 | 506.23 | 0.85 | 0.864 | *** | 76.80 | 0.86 | 0.867 | |
| Norway | 2698.10 | 0.97 | 681.68 | 1.15 | 1.184 | *** | 106.62 | 1.19 | 1.225 | * |
| Poland | 2615.00 | 0.94 | 447.27 | 0.75 | 0.802 | *** | 50.91 | 0.57 | 0.604 | *** |
| Hong Kong | 2501.14 | 0.90 | 427.44 | 0.72 | 0.801 | *** | 67.79 | 0.76 | 0.840 | |
| Malaysia | 2382.63 | 0.86 | 439.15 | 0.74 | 0.864 | *** | 56.03 | 0.63 | 0.729 | ** |
| Denmark | 2342.25 | 0.84 | 524.21 | 0.88 | 1.049 | | 91.48 | 1.02 | 1.211 | * |
| Portugal | 2113.47 | 0.76 | 411.25 | 0.69 | 0.912 | * | 68.48 | 0.76 | 1.004 | |
| Austria | 2009.23 | 0.72 | 525.28 | 0.89 | 1.225 | *** | 85.64 | 0.96 | 1.321 | ** |
| Finland | 1914.37 | 0.69 | 451.13 | 0.76 | 1.104 | ** | 55.67 | 0.62 | 0.902 | |
| Russia | 1897.00 | 0.68 | 331.50 | 0.56 | 0.819 | *** | 48.10 | 0.54 | 0.786 | * |
| New Zealand | 1704.37 | 0.61 | 336.39 | 0.57 | 0.925 | | 47.04 | 0.53 | 0.856 | |
| Israel | 1584.17 | 0.57 | 405.94 | 0.69 | 1.201 | *** | 70.75 | 0.79 | 1.385 | ** |
| Iran | 1541.01 | 0.55 | 430.64 | 0.73 | 1.310 | *** | 65.57 | 0.73 | 1.319 | * |
| Singapore | 1505.08 | 0.54 | 282.97 | 0.48 | 0.881 | ** | 52.58 | 0.59 | 1.083 | |
| Mexico | 1218.65 | 0.44 | 293.52 | 0.50 | 1.129 | * | 35.98 | 0.40 | 0.915 | |
| Czechia | 1216.97 | 0.44 | 266.20 | 0.45 | 1.025 | | 45.40 | 0.51 | 1.157 | |
| Hungary | 752.07 | 0.27 | 173.57 | 0.29 | 1.082 | | 23.15 | 0.26 | 0.954 | |
| Egypt | 328.04 | 0.12 | 47.80 | 0.08 | 0.683 | ** | 5.16 | 0.06 | 0.488 | * |
| *Total* | 256076.61 | 92.22 | 55185.09 | 93.14 | – | – | 8482.12 | 94.69 | – | – |

* $p < 0.05$, ** $p < 0.01$, *** $p < 0.001$

Table S19: Statistics about the production of Sociology papers in the 2010s for 38 countries/regions.

| | All papers | | Novel papers | | | | Atypical papers | | | |
|---|---|---|---|---|---|---|---|---|---|---|
| Country/region | Count | % | Count | % | $r_N$ | $p$-val | Count | % | $r_A$ | $p$-val |
| US | 78952.48 | 30.75 | 17133.33 | 31.92 | 1.038 | *** | 777.76 | 37.93 | 1.233 | *** |
| UK | 43674.75 | 17.01 | 8750.41 | 16.30 | 0.958 | *** | 295.43 | 14.41 | 0.847 | *** |
| Australia | 18773.04 | 7.31 | 3989.97 | 7.43 | 1.016 | | 91.47 | 4.46 | 0.610 | *** |
| Canada | 15467.96 | 6.03 | 3397.61 | 6.33 | 1.050 | *** | 85.79 | 4.18 | 0.694 | *** |
| South Africa | 6729.01 | 2.62 | 1417.86 | 2.64 | 1.008 | | 15.32 | 0.75 | 0.285 | *** |
| Germany | 6336.25 | 2.47 | 1347.53 | 2.51 | 1.017 | | 61.65 | 3.01 | 1.218 | |
| Sweden | 5864.67 | 2.28 | 1177.73 | 2.19 | 0.960 | | 43.07 | 2.10 | 0.920 | |
| Netherlands | 5756.27 | 2.24 | 1314.28 | 2.45 | 1.092 | *** | 46.60 | 2.27 | 1.014 | |
| Brazil | 5567.55 | 2.17 | 1174.15 | 2.19 | 1.009 | | 55.08 | 2.69 | 1.239 | |
| Spain | 5200.06 | 2.03 | 1023.36 | 1.91 | 0.941 | * | 43.60 | 2.13 | 1.050 | |
| France | 3724.93 | 1.45 | 824.06 | 1.54 | 1.058 | * | 33.64 | 1.64 | 1.131 | |
| New Zealand | 3683.39 | 1.43 | 728.99 | 1.36 | 0.946 | * | 25.16 | 1.23 | 0.855 | |
| Italy | 3651.71 | 1.42 | 823.77 | 1.53 | 1.079 | ** | 35.11 | 1.71 | 1.204 | |
| Denmark | 3253.74 | 1.27 | 611.06 | 1.14 | 0.898 | ** | 15.26 | 0.74 | 0.587 | * |
| Norway | 3068.60 | 1.20 | 585.22 | 1.09 | 0.912 | ** | 20.08 | 0.98 | 0.819 | |
| Finland | 3007.00 | 1.17 | 503.98 | 0.94 | 0.802 | *** | 22.87 | 1.12 | 0.952 | |
| Israel | 2878.22 | 1.12 | 519.10 | 0.97 | 0.862 | *** | 14.01 | 0.68 | 0.610 | * |
| Belgium | 2469.47 | 0.96 | 472.08 | 0.88 | 0.914 | * | 27.71 | 1.35 | 1.405 | * |
| China | 2366.64 | 0.92 | 556.25 | 1.04 | 1.124 | ** | 39.22 | 1.91 | 2.075 | *** |
| Hong Kong | 2277.26 | 0.89 | 394.28 | 0.73 | 0.828 | *** | 20.92 | 1.02 | 1.150 | |
| Switzerland | 1990.81 | 0.78 | 472.70 | 0.88 | 1.135 | ** | 20.64 | 1.01 | 1.298 | |
| India | 1813.77 | 0.71 | 379.53 | 0.71 | 1.001 | | 11.70 | 0.57 | 0.807 | |
| Turkey | 1511.67 | 0.59 | 240.41 | 0.45 | 0.761 | *** | 17.12 | 0.84 | 1.418 | |
| Portugal | 1510.20 | 0.59 | 270.09 | 0.50 | 0.855 | ** | 8.60 | 0.42 | 0.713 | |
| Singapore | 1430.89 | 0.56 | 227.60 | 0.42 | 0.761 | *** | 11.22 | 0.55 | 0.982 | |
| Japan | 1333.43 | 0.52 | 322.64 | 0.60 | 1.157 | ** | 9.95 | 0.49 | 0.934 | |
| Malaysia | 1146.35 | 0.45 | 262.73 | 0.49 | 1.096 | * | 6.08 | 0.30 | 0.664 | |
| Mexico | 1142.61 | 0.45 | 258.73 | 0.48 | 1.083 | | 8.85 | 0.43 | 0.970 | |
| Korea | 1112.13 | 0.43 | 224.96 | 0.42 | 0.967 | | 9.61 | 0.47 | 1.082 | |
| Poland | 1106.03 | 0.43 | 242.42 | 0.45 | 1.048 | | 10.44 | 0.51 | 1.182 | |
| Austria | 1057.49 | 0.41 | 238.59 | 0.44 | 1.079 | | 8.54 | 0.42 | 1.011 | |
| Taiwan | 1013.12 | 0.39 | 223.76 | 0.42 | 1.056 | | 16.37 | 0.80 | 2.023 | ** |
| Iran | 887.98 | 0.35 | 237.63 | 0.44 | 1.280 | *** | 15.12 | 0.74 | 2.133 | ** |
| Russia | 821.41 | 0.32 | 189.38 | 0.35 | 1.103 | | 6.17 | 0.30 | 0.941 | |
| Greece | 771.37 | 0.30 | 161.59 | 0.30 | 1.002 | | 10.95 | 0.53 | 1.777 | * |
| Hungary | 517.45 | 0.20 | 104.01 | 0.19 | 0.961 | | 5.10 | 0.25 | 1.234 | |
| Czechia | 486.72 | 0.19 | 95.39 | 0.18 | 0.937 | | 1.00 | 0.05 | 0.257 | |
| Egypt | 216.11 | 0.08 | 37.97 | 0.07 | 0.840 | | 1.50 | 0.07 | 0.869 | |
| *Total* | 242572.54 | 94.49 | 50935.16 | 94.88 | – | – | 1948.71 | 95.04 | – | – |

* $p < 0.05$, ** $p < 0.01$, *** $p < 0.001$

Table S20: Statistics about the production of Business papers in the 2010s for 38 countries/regions.

| | All papers | | Novel papers | | | | Atypical papers | | | |
|---|---|---|---|---|---|---|---|---|---|---|
| Country/region | Count | % | Count | % | $r_N$ | $p$-val | Count | % | $r_A$ | $p$-val |
| US | 52761.58 | 24.40 | 15820.77 | 25.69 | 1.053 | *** | 1629.05 | 26.21 | 1.074 | *** |
| UK | 16812.14 | 7.78 | 5229.44 | 8.49 | 1.092 | *** | 462.07 | 7.43 | 0.956 | |
| China | 12330.70 | 5.70 | 3916.68 | 6.36 | 1.115 | *** | 563.69 | 9.07 | 1.590 | *** |
| Australia | 11425.16 | 5.28 | 3565.00 | 5.79 | 1.095 | *** | 277.51 | 4.46 | 0.845 | ** |
| Germany | 7392.39 | 3.42 | 2130.92 | 3.46 | 1.012 | | 256.44 | 4.13 | 1.207 | ** |
| Canada | 7339.10 | 3.39 | 2376.19 | 3.86 | 1.137 | *** | 222.31 | 3.58 | 1.054 | |
| India | 6820.63 | 3.15 | 1609.01 | 2.61 | 0.828 | *** | 138.80 | 2.23 | 0.708 | *** |
| Spain | 6597.00 | 3.05 | 1429.78 | 2.32 | 0.761 | *** | 203.17 | 3.27 | 1.071 | |
| Italy | 5850.20 | 2.71 | 1715.26 | 2.79 | 1.029 | | 196.99 | 3.17 | 1.171 | * |
| Netherlands | 5240.91 | 2.42 | 1910.12 | 3.10 | 1.280 | *** | 166.78 | 2.68 | 1.107 | |
| Taiwan | 4584.73 | 2.12 | 888.54 | 1.44 | 0.680 | *** | 118.58 | 1.91 | 0.900 | |
| Korea | 4005.76 | 1.85 | 835.26 | 1.36 | 0.732 | *** | 96.32 | 1.55 | 0.836 | * |
| Brazil | 3965.69 | 1.83 | 1250.31 | 2.03 | 1.107 | *** | 103.57 | 1.67 | 0.908 | |
| France | 3828.29 | 1.77 | 959.68 | 1.56 | 0.880 | *** | 132.62 | 2.13 | 1.205 | * |
| Malaysia | 3744.60 | 1.73 | 778.72 | 1.26 | 0.730 | *** | 61.02 | 0.98 | 0.567 | *** |
| Sweden | 3664.11 | 1.69 | 996.49 | 1.62 | 0.955 | * | 106.34 | 1.71 | 1.009 | |
| South Africa | 3373.25 | 1.56 | 1042.84 | 1.69 | 1.085 | *** | 62.28 | 1.00 | 0.642 | *** |
| Finland | 2943.50 | 1.36 | 651.95 | 1.06 | 0.778 | *** | 70.56 | 1.14 | 0.834 | |
| Japan | 2936.80 | 1.36 | 916.20 | 1.49 | 1.095 | *** | 103.21 | 1.66 | 1.222 | * |
| Hong Kong | 2429.83 | 1.12 | 449.85 | 0.73 | 0.650 | *** | 55.91 | 0.90 | 0.800 | * |
| Poland | 2311.70 | 1.07 | 484.19 | 0.79 | 0.735 | *** | 43.65 | 0.70 | 0.657 | ** |
| Turkey | 2259.84 | 1.05 | 490.19 | 0.80 | 0.762 | *** | 42.39 | 0.68 | 0.652 | ** |
| Switzerland | 2233.39 | 1.03 | 762.37 | 1.24 | 1.198 | *** | 73.98 | 1.19 | 1.152 | |
| Iran | 2099.64 | 0.97 | 636.36 | 1.03 | 1.064 | * | 58.46 | 0.94 | 0.968 | |
| Norway | 1964.53 | 0.91 | 558.67 | 0.91 | 0.998 | | 59.96 | 0.96 | 1.062 | |
| Portugal | 1889.08 | 0.87 | 472.20 | 0.77 | 0.878 | *** | 63.54 | 1.02 | 1.170 | |
| Denmark | 1879.77 | 0.87 | 551.39 | 0.90 | 1.030 | | 80.92 | 1.30 | 1.497 | *** |
| New Zealand | 1873.31 | 0.87 | 504.46 | 0.82 | 0.945 | | 42.97 | 0.69 | 0.798 | |
| Belgium | 1750.93 | 0.81 | 574.39 | 0.93 | 1.152 | *** | 69.24 | 1.11 | 1.375 | ** |
| Greece | 1547.55 | 0.72 | 397.21 | 0.65 | 0.901 | ** | 35.62 | 0.57 | 0.801 | |
| Austria | 1175.31 | 0.54 | 375.36 | 0.61 | 1.121 | ** | 37.19 | 0.60 | 1.101 | |
| Singapore | 1094.28 | 0.51 | 295.00 | 0.48 | 0.946 | | 35.98 | 0.58 | 1.144 | |
| Russia | 1057.57 | 0.49 | 213.41 | 0.35 | 0.708 | *** | 25.55 | 0.41 | 0.840 | |
| Mexico | 1010.26 | 0.47 | 350.28 | 0.57 | 1.217 | *** | 23.28 | 0.37 | 0.801 | |
| Czechia | 840.61 | 0.39 | 229.08 | 0.37 | 0.957 | | 13.83 | 0.22 | 0.572 | * |
| Israel | 727.44 | 0.34 | 232.02 | 0.38 | 1.120 | * | 23.32 | 0.38 | 1.115 | |
| Egypt | 451.29 | 0.21 | 73.43 | 0.12 | 0.571 | *** | 6.39 | 0.10 | 0.493 | * |
| Hungary | 403.04 | 0.19 | 122.27 | 0.20 | 1.065 | | 9.34 | 0.15 | 0.806 | |
| *Total* | 194615.90 | 90.02 | 55795.32 | 90.61 | – | – | 5772.85 | 92.87 | – | – |

* $p < 0.05$, ** $p < 0.01$, *** $p < 0.001$

Table S21: Statistics about the production of Geography papers in the 2010s for 38 countries/regions.

| | All papers | | Novel papers | | | | Atypical papers | | | |
|---|---|---|---|---|---|---|---|---|---|---|
| Country/region | Count | % | Count | % | $r_N$ | $p$-val | Count | % | $r_A$ | $p$-val |
| US | 40601.81 | 25.38 | 17008.85 | 27.04 | 1.066 | *** | 2228.52 | 29.66 | 1.169 | *** |
| UK | 9836.16 | 6.15 | 4192.93 | 6.67 | 1.084 | *** | 478.69 | 6.37 | 1.036 | |
| China | 8153.59 | 5.10 | 3930.30 | 6.25 | 1.226 | *** | 506.59 | 6.74 | 1.323 | *** |
| Australia | 7787.06 | 4.87 | 3126.90 | 4.97 | 1.021 | | 345.48 | 4.60 | 0.945 | |
| Brazil | 7666.92 | 4.79 | 2541.78 | 4.04 | 0.843 | *** | 251.81 | 3.35 | 0.699 | *** |
| Canada | 6700.61 | 4.19 | 2578.62 | 4.10 | 0.979 | | 338.31 | 4.50 | 1.075 | |
| Spain | 6334.86 | 3.96 | 2014.44 | 3.20 | 0.809 | *** | 295.38 | 3.93 | 0.993 | |
| Germany | 4992.07 | 3.12 | 1981.31 | 3.15 | 1.010 | | 267.75 | 3.56 | 1.142 | * |
| India | 4924.18 | 3.08 | 1981.46 | 3.15 | 1.024 | | 210.86 | 2.81 | 0.912 | |
| Italy | 4277.82 | 2.67 | 1627.21 | 2.59 | 0.968 | * | 207.32 | 2.76 | 1.032 | |
| France | 4184.87 | 2.62 | 1510.59 | 2.40 | 0.918 | *** | 242.19 | 3.22 | 1.232 | *** |
| South Africa | 3462.39 | 2.16 | 1187.90 | 1.89 | 0.873 | *** | 90.90 | 1.21 | 0.559 | *** |
| Mexico | 3028.82 | 1.89 | 937.37 | 1.49 | 0.787 | *** | 77.45 | 1.03 | 0.545 | *** |
| Japan | 2701.60 | 1.69 | 1026.28 | 1.63 | 0.966 | | 106.30 | 1.41 | 0.838 | * |
| Netherlands | 2117.51 | 1.32 | 891.59 | 1.42 | 1.071 | ** | 110.92 | 1.48 | 1.115 | |
| Poland | 1810.76 | 1.13 | 484.78 | 0.77 | 0.681 | *** | 48.16 | 0.64 | 0.566 | *** |
| Sweden | 1789.27 | 1.12 | 701.42 | 1.12 | 0.997 | | 86.85 | 1.16 | 1.034 | |
| Russia | 1624.65 | 1.02 | 346.50 | 0.55 | 0.543 | *** | 37.89 | 0.50 | 0.497 | *** |
| Portugal | 1589.13 | 0.99 | 541.74 | 0.86 | 0.867 | *** | 76.28 | 1.02 | 1.022 | |
| Iran | 1553.14 | 0.97 | 652.34 | 1.04 | 1.068 | * | 75.11 | 1.00 | 1.030 | |
| Switzerland | 1505.75 | 0.94 | 602.68 | 0.96 | 1.018 | | 82.97 | 1.10 | 1.173 | |
| Korea | 1421.27 | 0.89 | 568.97 | 0.90 | 1.018 | | 71.60 | 0.95 | 1.073 | |
| New Zealand | 1413.38 | 0.88 | 543.35 | 0.86 | 0.978 | | 54.54 | 0.73 | 0.822 | |
| Norway | 1283.25 | 0.80 | 480.00 | 0.76 | 0.951 | | 65.84 | 0.88 | 1.093 | |
| Belgium | 1206.64 | 0.75 | 514.05 | 0.82 | 1.084 | * | 57.88 | 0.77 | 1.021 | |
| Turkey | 1195.45 | 0.75 | 377.60 | 0.60 | 0.803 | *** | 51.43 | 0.68 | 0.916 | |
| Czechia | 1019.72 | 0.64 | 274.35 | 0.44 | 0.684 | *** | 37.48 | 0.50 | 0.783 | |
| Finland | 1017.52 | 0.64 | 361.99 | 0.58 | 0.905 | ** | 41.73 | 0.56 | 0.873 | |
| Denmark | 971.36 | 0.61 | 384.39 | 0.61 | 1.007 | | 57.56 | 0.77 | 1.262 | * |
| Greece | 921.09 | 0.58 | 352.32 | 0.56 | 0.973 | | 50.94 | 0.68 | 1.178 | |
| Malaysia | 874.24 | 0.55 | 392.15 | 0.62 | 1.141 | *** | 36.14 | 0.48 | 0.880 | |
| Austria | 748.75 | 0.47 | 324.91 | 0.52 | 1.104 | * | 43.80 | 0.58 | 1.246 | |
| Hong Kong | 743.21 | 0.46 | 375.47 | 0.60 | 1.285 | *** | 38.77 | 0.52 | 1.111 | |
| Israel | 735.47 | 0.46 | 311.02 | 0.49 | 1.076 | | 30.31 | 0.40 | 0.878 | |
| Taiwan | 717.32 | 0.45 | 336.85 | 0.54 | 1.195 | *** | 51.45 | 0.68 | 1.527 | ** |
| Hungary | 435.12 | 0.27 | 137.40 | 0.22 | 0.803 | *** | 13.38 | 0.18 | 0.655 | |
| Singapore | 389.35 | 0.24 | 186.09 | 0.30 | 1.216 | *** | 16.31 | 0.22 | 0.892 | |
| Egypt | 297.86 | 0.19 | 123.88 | 0.20 | 1.058 | | 12.01 | 0.16 | 0.858 | |
| *Total* | 142033.99 | 88.78 | 55911.76 | 88.90 | – | – | 6896.91 | 91.80 | – | – |

* $p < 0.05$, ** $p < 0.01$, *** $p < 0.001$

Table S22: Statistics about the production of Political Science papers in the 2010s for 38 countries/regions.

| | All papers | | Novel papers | | | | Atypical papers | | | |
|---|---|---|---|---|---|---|---|---|---|---|
| Country/region | Count | % | Count | % | $r_N$ | $p$-val | Count | % | $r_A$ | $p$-val |
| US | 38224.93 | 27.79 | 9212.73 | 28.95 | 1.042 | *** | 636.26 | 33.38 | 1.201 | *** |
| UK | 16184.45 | 11.76 | 3605.67 | 11.33 | 0.963 | ** | 204.73 | 10.74 | 0.913 | |
| Germany | 7731.15 | 5.62 | 1805.26 | 5.67 | 1.009 | | 103.69 | 5.44 | 0.968 | |
| Canada | 7282.62 | 5.29 | 1842.81 | 5.79 | 1.094 | *** | 68.74 | 3.61 | 0.681 | *** |
| Australia | 7066.30 | 5.14 | 1682.52 | 5.29 | 1.029 | | 62.81 | 3.30 | 0.642 | *** |
| France | 5123.24 | 3.72 | 1533.20 | 4.82 | 1.294 | *** | 122.13 | 6.41 | 1.720 | *** |
| Brazil | 4502.53 | 3.27 | 1035.29 | 3.25 | 0.994 | | 57.14 | 3.00 | 0.916 | |
| Spain | 4427.80 | 3.22 | 930.74 | 2.92 | 0.909 | *** | 86.92 | 4.56 | 1.417 | *** |
| Netherlands | 3314.69 | 2.41 | 776.95 | 2.44 | 1.013 | | 41.23 | 2.16 | 0.898 | |
| South Africa | 2737.83 | 1.99 | 688.98 | 2.16 | 1.088 | ** | 23.15 | 1.21 | 0.610 | ** |
| Sweden | 2256.57 | 1.64 | 486.81 | 1.53 | 0.933 | * | 21.54 | 1.13 | 0.689 | |
| Italy | 2138.46 | 1.55 | 425.57 | 1.34 | 0.860 | *** | 33.13 | 1.74 | 1.118 | |
| China | 1941.74 | 1.41 | 525.11 | 1.65 | 1.169 | *** | 45.05 | 2.36 | 1.674 | *** |
| Switzerland | 1784.59 | 1.30 | 431.87 | 1.36 | 1.046 | | 23.54 | 1.23 | 0.952 | |
| Belgium | 1688.03 | 1.23 | 340.15 | 1.07 | 0.871 | ** | 24.72 | 1.30 | 1.057 | |
| Norway | 1675.54 | 1.22 | 326.95 | 1.03 | 0.843 | *** | 21.19 | 1.11 | 0.913 | |
| Mexico | 1558.81 | 1.13 | 303.68 | 0.95 | 0.842 | *** | 12.69 | 0.67 | 0.587 | * |
| Denmark | 1374.48 | 1.00 | 238.49 | 0.75 | 0.750 | *** | 22.15 | 1.16 | 1.163 | |
| India | 1267.30 | 0.92 | 317.00 | 1.00 | 1.081 | | 16.79 | 0.88 | 0.956 | |
| Hong Kong | 1203.87 | 0.88 | 190.36 | 0.60 | 0.684 | *** | 7.28 | 0.38 | 0.437 | ** |
| Israel | 1154.98 | 0.84 | 208.04 | 0.65 | 0.779 | *** | 5.28 | 0.28 | 0.330 | ** |
| Japan | 1140.86 | 0.83 | 262.94 | 0.83 | 0.996 | | 18.88 | 0.99 | 1.194 | |
| Finland | 1124.21 | 0.82 | 232.11 | 0.73 | 0.892 | * | 11.59 | 0.61 | 0.744 | |
| New Zealand | 1111.96 | 0.81 | 270.21 | 0.85 | 1.050 | | 9.33 | 0.49 | 0.606 | |
| Korea | 1097.91 | 0.80 | 215.30 | 0.68 | 0.848 | ** | 19.42 | 1.02 | 1.277 | |
| Portugal | 1001.10 | 0.73 | 235.06 | 0.74 | 1.015 | | 16.40 | 0.86 | 1.182 | |
| Turkey | 996.29 | 0.72 | 137.24 | 0.43 | 0.595 | *** | 8.05 | 0.42 | 0.583 | |
| Austria | 885.93 | 0.64 | 185.64 | 0.58 | 0.906 | | 16.36 | 0.86 | 1.332 | |
| Poland | 881.12 | 0.64 | 136.22 | 0.43 | 0.668 | *** | 6.50 | 0.34 | 0.532 | |
| Singapore | 716.88 | 0.52 | 125.19 | 0.39 | 0.755 | *** | 5.53 | 0.29 | 0.557 | |
| Russia | 681.67 | 0.50 | 136.46 | 0.43 | 0.865 | * | 10.31 | 0.54 | 1.092 | |
| Malaysia | 498.97 | 0.36 | 123.72 | 0.39 | 1.072 | | 7.02 | 0.37 | 1.016 | |
| Czechia | 466.59 | 0.34 | 81.03 | 0.25 | 0.751 | ** | 3.95 | 0.21 | 0.611 | |
| Greece | 442.05 | 0.32 | 95.26 | 0.30 | 0.932 | | 6.21 | 0.33 | 1.014 | |
| Taiwan | 439.22 | 0.32 | 106.34 | 0.33 | 1.047 | | 8.51 | 0.45 | 1.398 | |
| Hungary | 376.72 | 0.27 | 62.29 | 0.20 | 0.715 | *** | 4.43 | 0.23 | 0.849 | |
| Iran | 259.37 | 0.19 | 101.50 | 0.32 | 1.692 | *** | 5.42 | 0.28 | 1.508 | |
| Egypt | 134.39 | 0.10 | 22.46 | 0.07 | 0.722 | * | 0.50 | 0.03 | 0.269 | |
| *Total* | 126895.15 | 92.24 | 29437.16 | 92.49 | – | – | 1798.62 | 94.35 | – | – |

* $p < 0.05$, ** $p < 0.01$, *** $p < 0.001$

Table S23: Statistics about the production of science and novel and atypical science in the 2010s by US.

| Discipline | All papers | Novel papers | | | Atypical papers | | |
|---|---|---|---|---|---|---|---|
| | | Count | $r_N$ | $p$-val | Count | $r_A$ | $p$-val |
| Medicine | 1014773 | 435542 | 1.003 | *** | 73212 | 1.185 | *** |
| Biology | 584165 | 237632 | 0.929 | *** | 61714 | 1.228 | *** |
| Psychology | 321580 | 100057 | 0.954 | *** | 16111 | 1.069 | *** |
| Chemistry | 289137 | 150847 | 1.010 | *** | 50443 | 1.186 | *** |
| Materials science | 261441 | 120695 | 1.151 | *** | 43548 | 1.203 | *** |
| Computer science | 161711 | 74885 | 1.141 | *** | 14093 | 1.270 | *** |
| Physics | 127700 | 33838 | 1.067 | *** | 16802 | 1.169 | *** |
| Mathematics | 115329 | 36525 | 1.172 | *** | 8240 | 1.280 | *** |
| Environmental science | 94381 | 38264 | 0.987 | *** | 14160 | 1.138 | *** |
| Sociology | 78952 | 17133 | 1.038 | *** | 778 | 1.233 | *** |
| Economics | 74394 | 16421 | 1.034 | *** | 2634 | 1.098 | *** |
| Engineering | 69264 | 26845 | 1.209 | *** | 4759 | 1.218 | *** |
| Geology | 68117 | 16607 | 1.054 | *** | 7842 | 1.264 | *** |
| Business | 52762 | 15821 | 1.053 | *** | 1629 | 1.074 | *** |
| Geography | 40602 | 17009 | 1.066 | *** | 2229 | 1.169 | *** |
| Political science | 38225 | 9213 | 1.042 | *** | 636 | 1.201 | *** |

Table S24: Statistics about the production of science and novel and atypical science in the 2010s by China.

| Discipline | All papers | Novel papers | | | Atypical papers | | |
|---|---|---|---|---|---|---|---|
| | | Count | $r_N$ | $p$-val | Count | $r_A$ | $p$-val |
| Materials science | 462187 | 159845 | 0.862 | *** | 71607 | 1.119 | *** |
| Chemistry | 351994 | 175023 | 0.963 | *** | 58529 | 1.131 | *** |
| Biology | 244355 | 125376 | 1.172 | *** | 18514 | 0.881 | *** |
| Medicine | 209529 | 109504 | 1.221 | *** | 11262 | 0.883 | *** |
| Computer science | 151358 | 56161 | 0.914 | *** | 11128 | 1.071 | *** |
| Mathematics | 120867 | 28797 | 0.881 | *** | 6870 | 1.018 | * |
| Engineering | 84874 | 23683 | 0.870 | *** | 3803 | 0.794 | *** |
| Physics | 72307 | 17532 | 0.977 | *** | 7701 | 0.947 | *** |
| Environmental science | 46305 | 19573 | 1.029 | *** | 6734 | 1.103 | *** |
| Geology | 39059 | 8380 | 0.928 | *** | 2718 | 0.764 | *** |
| Psychology | 18055 | 6888 | 1.169 | *** | 1445 | 1.708 | *** |
| Economics | 13758 | 3785 | 1.289 | *** | 855 | 1.927 | *** |
| Business | 12331 | 3917 | 1.115 | *** | 564 | 1.590 | *** |
| Geography | 8154 | 3930 | 1.226 | *** | 507 | 1.323 | *** |
| Sociology | 2367 | 556 | 1.124 | ** | 39 | 2.075 | *** |
| Political science | 1942 | 525 | 1.169 | *** | 45 | 1.674 | *** |

Table S25: Statistics about the production of science and novel and atypical science in the 2010s by UK.

| Discipline | All papers | Novel papers Count | $r_N$ | $p$-val | Atypical papers Count | $r_A$ | $p$-val |
|---|---|---|---|---|---|---|---|
| Medicine | 237069 | 98296 | 0.969 | *** | 14833 | 1.028 | *** |
| Biology | 105020 | 43786 | 0.952 | *** | 10519 | 1.165 | *** |
| Psychology | 75382 | 26369 | 1.072 | *** | 3556 | 1.007 | |
| Chemistry | 56143 | 28671 | 0.989 | ** | 8941 | 1.083 | *** |
| Materials science | 51621 | 23842 | 1.151 | *** | 7294 | 1.020 | * |
| Sociology | 43675 | 8750 | 0.958 | *** | 295 | 0.847 | *** |
| Computer science | 39805 | 18334 | 1.135 | *** | 2971 | 1.088 | *** |
| Physics | 30331 | 7577 | 1.006 | | 3628 | 1.063 | *** |
| Mathematics | 25289 | 8076 | 1.181 | *** | 1662 | 1.177 | *** |
| Economics | 25067 | 5459 | 1.021 | * | 656 | 0.811 | *** |
| Engineering | 21037 | 8091 | 1.199 | *** | 1361 | 1.147 | *** |
| Business | 16812 | 5229 | 1.092 | *** | 462 | 0.956 | |
| Geology | 16205 | 3800 | 1.014 | | 1604 | 1.087 | *** |
| Political science | 16184 | 3606 | 0.963 | ** | 205 | 0.913 | |
| Environmental science | 15725 | 6672 | 1.033 | *** | 2167 | 1.045 | * |
| Geography | 9836 | 4193 | 1.084 | *** | 479 | 1.036 | |

Table S26: Statistics about the production of science and novel and atypical science in the 2010s by France.

| Discipline | All papers | Novel papers Count | $r_N$ | $p$-val | Atypical papers Count | $r_A$ | $p$-val |
|---|---|---|---|---|---|---|---|
| Medicine | 109053 | 39492 | 0.846 | *** | 7035 | 1.060 | *** |
| Biology | 69757 | 27541 | 0.902 | *** | 6576 | 1.096 | *** |
| Chemistry | 50511 | 24948 | 0.956 | *** | 8048 | 1.084 | *** |
| Materials science | 47789 | 20853 | 1.088 | *** | 6740 | 1.018 | |
| Mathematics | 29481 | 8273 | 1.038 | *** | 1559 | 0.947 | * |
| Physics | 25419 | 7242 | 1.148 | *** | 3447 | 1.205 | *** |
| Computer science | 22663 | 9372 | 1.019 | ** | 1690 | 1.087 | *** |
| Psychology | 15784 | 5295 | 1.028 | ** | 926 | 1.253 | *** |
| Geology | 12331 | 2864 | 1.004 | | 1387 | 1.236 | *** |
| Engineering | 11359 | 4022 | 1.104 | *** | 720 | 1.123 | *** |
| Environmental science | 9638 | 3708 | 0.937 | *** | 1390 | 1.094 | *** |
| Economics | 8080 | 1525 | 0.885 | *** | 289 | 1.108 | * |
| Political science | 5123 | 1533 | 1.294 | *** | 122 | 1.720 | *** |
| Geography | 4185 | 1511 | 0.918 | *** | 242 | 1.232 | *** |
| Business | 3828 | 960 | 0.880 | *** | 133 | 1.205 | * |
| Sociology | 3725 | 824 | 1.058 | * | 34 | 1.131 | |

Table S27: Statistics about the production of science and novel and atypical science in the 2010s by Germany.

| Discipline | All papers | Novel papers Count | $r_N$ | $p$-val | Atypical papers Count | $r_A$ | $p$-val |
|---|---|---|---|---|---|---|---|
| Medicine | 131316 | 53606 | 0.954 | *** | 9496 | 1.188 | *** |
| Biology | 103984 | 42085 | 0.925 | *** | 9603 | 1.074 | *** |
| Chemistry | 85600 | 40930 | 0.926 | *** | 13194 | 1.048 | *** |
| Materials science | 72932 | 30252 | 1.034 | *** | 9919 | 0.982 | * |
| Physics | 40256 | 9232 | 0.924 | *** | 4708 | 1.040 | ** |
| Psychology | 38190 | 12453 | 1.000 | | 2544 | 1.422 | *** |
| Computer science | 32098 | 13819 | 1.061 | *** | 2634 | 1.196 | *** |
| Mathematics | 28114 | 7702 | 1.013 | | 1604 | 1.022 | |
| Economics | 14698 | 3021 | 0.963 | ** | 498 | 1.050 | |
| Engineering | 13964 | 4747 | 1.060 | *** | 794 | 1.008 | |
| Environmental science | 13825 | 5508 | 0.970 | ** | 2069 | 1.135 | *** |
| Geology | 13054 | 3175 | 1.052 | *** | 1444 | 1.215 | *** |
| Political science | 7731 | 1805 | 1.009 | | 104 | 0.968 | |
| Business | 7392 | 2131 | 1.012 | | 256 | 1.207 | ** |
| Sociology | 6336 | 1348 | 1.017 | | 62 | 1.218 | |
| Geography | 4992 | 1981 | 1.010 | | 268 | 1.142 | * |

Table S28: Statistics about the production of science and novel and atypical science in the 2010s by Canada.

| Discipline | All papers | Novel papers Count | $r_N$ | $p$-val | Atypical papers Count | $r_A$ | $p$-val |
|---|---|---|---|---|---|---|---|
| Medicine | 120200 | 52092 | 1.013 | *** | 7408 | 1.012 | |
| Biology | 67634 | 27335 | 0.923 | *** | 6378 | 1.096 | *** |
| Psychology | 44418 | 14189 | 0.979 | *** | 2061 | 0.990 | |
| Chemistry | 36841 | 18796 | 0.988 | ** | 5645 | 1.042 | *** |
| Materials science | 29073 | 13332 | 1.143 | *** | 4320 | 1.073 | *** |
| Computer science | 24041 | 9697 | 0.994 | | 1866 | 1.131 | *** |
| Mathematics | 18251 | 5332 | 1.081 | *** | 1242 | 1.219 | *** |
| Sociology | 15468 | 3398 | 1.050 | *** | 86 | 0.694 | *** |
| Environmental science | 14278 | 5597 | 0.955 | *** | 1952 | 1.037 | * |
| Engineering | 13625 | 4465 | 1.022 | * | 910 | 1.183 | *** |
| Physics | 12432 | 3255 | 1.055 | *** | 1573 | 1.124 | *** |
| Geology | 11279 | 2634 | 1.009 | | 1107 | 1.077 | ** |
| Economics | 9278 | 2034 | 1.027 | | 307 | 1.026 | |
| Business | 7339 | 2376 | 1.137 | *** | 222 | 1.054 | |
| Political science | 7283 | 1843 | 1.094 | *** | 69 | 0.681 | *** |
| Geography | 6701 | 2579 | 0.979 | | 338 | 1.075 | |

Table S29: Statistics about the production of science and novel and atypical science in the 2010s by Italy.

| Discipline | All papers | Novel papers Count | $r_N$ | $p$-val | Atypical papers Count | $r_A$ | $p$-val |
|---|---|---|---|---|---|---|---|
| Medicine | 129026 | 48033 | 0.870 | *** | 7609 | 0.969 | ** |
| Biology | 59171 | 28318 | 1.093 | *** | 4362 | 0.857 | *** |
| Chemistry | 43129 | 24576 | 1.103 | *** | 5740 | 0.905 | *** |
| Materials science | 33434 | 15446 | 1.151 | *** | 4365 | 0.943 | *** |
| Computer science | 24287 | 10487 | 1.064 | *** | 1660 | 0.996 | |
| Mathematics | 21599 | 5942 | 1.018 | | 1128 | 0.936 | ** |
| Physics | 21522 | 5262 | 0.985 | | 2365 | 0.977 | |
| Psychology | 19167 | 6518 | 1.043 | *** | 1048 | 1.167 | *** |
| Engineering | 18140 | 5925 | 1.018 | * | 1139 | 1.113 | *** |
| Geology | 10700 | 2700 | 1.091 | *** | 1076 | 1.105 | *** |
| Environmental science | 9608 | 4318 | 1.095 | *** | 1294 | 1.022 | |
| Economics | 9406 | 1949 | 0.971 | | 275 | 0.908 | * |
| Business | 5850 | 1715 | 1.029 | | 197 | 1.171 | * |
| Geography | 4278 | 1627 | 0.968 | * | 207 | 1.032 | |
| Sociology | 3652 | 824 | 1.079 | ** | 35 | 1.204 | |
| Political science | 2138 | 426 | 0.860 | *** | 33 | 1.118 | |

Table S30: Statistics about the production of science and novel and atypical science in the 2010s by Australia.

| Discipline | All papers | Novel papers Count | $r_N$ | $p$-val | Atypical papers Count | $r_A$ | $p$-val |
|---|---|---|---|---|---|---|---|
| Medicine | 120333 | 51261 | 0.996 | | 6122 | 0.836 | *** |
| Biology | 60919 | 24627 | 0.924 | *** | 5312 | 1.014 | |
| Psychology | 43788 | 14429 | 1.010 | | 1477 | 0.720 | *** |
| Chemistry | 28031 | 15135 | 1.046 | *** | 4476 | 1.086 | *** |
| Materials science | 27930 | 12277 | 1.096 | *** | 4104 | 1.061 | *** |
| Sociology | 18773 | 3990 | 1.016 | | 91 | 0.610 | *** |
| Computer science | 18571 | 8113 | 1.076 | *** | 1280 | 1.004 | |
| Engineering | 12580 | 4464 | 1.106 | *** | 704 | 0.992 | |
| Economics | 12203 | 2859 | 1.098 | *** | 308 | 0.781 | *** |
| Environmental science | 11918 | 4975 | 1.017 | | 1526 | 0.972 | |
| Mathematics | 11493 | 3729 | 1.200 | *** | 791 | 1.233 | *** |
| Business | 11425 | 3565 | 1.095 | *** | 278 | 0.845 | ** |
| Geology | 10487 | 2478 | 1.022 | | 986 | 1.032 | |
| Physics | 8991 | 2409 | 1.079 | *** | 1083 | 1.070 | ** |
| Geography | 7787 | 3127 | 1.021 | | 345 | 0.945 | |
| Political science | 7066 | 1683 | 1.029 | | 63 | 0.642 | *** |

Table S31: Statistics about the production of science and novel and atypical science in the 2010s by Spain.

| Discipline | All papers | Novel papers | | | Atypical papers | | |
|---|---|---|---|---|---|---|---|
| | | Count | $r_N$ | $p$-val | Count | $r_A$ | $p$-val |
| Medicine | 103412 | 35340 | 0.799 | *** | 5176 | 0.822 | *** |
| Biology | 57934 | 23026 | 0.908 | *** | 4887 | 0.981 | |
| Chemistry | 47771 | 22052 | 0.894 | *** | 7346 | 1.046 | *** |
| Materials science | 28737 | 12275 | 1.065 | *** | 4241 | 1.065 | *** |
| Computer science | 25192 | 10836 | 1.060 | *** | 1496 | 0.865 | *** |
| Psychology | 20061 | 5797 | 0.886 | *** | 648 | 0.690 | *** |
| Mathematics | 19031 | 5218 | 1.014 | | 1062 | 1.000 | |
| Physics | 14266 | 3301 | 0.932 | *** | 1552 | 0.967 | |
| Engineering | 12718 | 4323 | 1.060 | *** | 860 | 1.198 | *** |
| Environmental science | 11440 | 4544 | 0.967 | ** | 1597 | 1.059 | ** |
| Economics | 8063 | 1541 | 0.896 | *** | 245 | 0.942 | |
| Geology | 6816 | 1613 | 1.023 | | 543 | 0.875 | *** |
| Business | 6597 | 1430 | 0.761 | *** | 203 | 1.071 | |
| Geography | 6335 | 2014 | 0.809 | *** | 295 | 0.993 | |
| Sociology | 5200 | 1023 | 0.941 | * | 44 | 1.050 | |
| Political science | 4428 | 931 | 0.909 | *** | 87 | 1.417 | *** |

Table S32: Statistics about the production of science and novel and atypical science in the 2010s by Korea.

| Discipline | All papers | Novel papers | | | Atypical papers | | |
|---|---|---|---|---|---|---|---|
| | | Count | $r_N$ | $p$-val | Count | $r_A$ | $p$-val |
| Medicine | 128598 | 51900 | 0.943 | *** | 7157 | 0.914 | *** |
| Materials science | 88239 | 33544 | 0.948 | *** | 13014 | 1.065 | *** |
| Chemistry | 57191 | 33204 | 1.124 | *** | 7429 | 0.883 | *** |
| Biology | 53852 | 27562 | 1.169 | *** | 4136 | 0.893 | *** |
| Computer science | 28778 | 9469 | 0.811 | *** | 1476 | 0.748 | *** |
| Engineering | 16613 | 4705 | 0.883 | *** | 768 | 0.819 | *** |
| Mathematics | 13726 | 3209 | 0.865 | *** | 811 | 1.058 | * |
| Physics | 11944 | 2718 | 0.917 | *** | 1140 | 0.848 | *** |
| Psychology | 11496 | 3967 | 1.058 | *** | 473 | 0.879 | ** |
| Environmental science | 6624 | 2577 | 0.948 | *** | 798 | 0.914 | ** |
| Business | 4006 | 835 | 0.732 | *** | 96 | 0.836 | * |
| Economics | 3962 | 657 | 0.777 | *** | 110 | 0.862 | |
| Geology | 3227 | 746 | 0.999 | | 260 | 0.886 | * |
| Geography | 1421 | 569 | 1.018 | | 72 | 1.073 | |
| Sociology | 1112 | 225 | 0.967 | | 10 | 1.082 | |
| Political science | 1098 | 215 | 0.848 | ** | 19 | 1.277 | |

Table S33: Statistics about the production of science and novel and atypical science in the 2010s by India.

| Discipline | All papers | Novel papers Count | $r_N$ | $p$-val | Atypical papers Count | $r_A$ | $p$-val |
|---|---|---|---|---|---|---|---|
| Chemistry | 112952 | 62173 | 1.066 | *** | 15761 | 0.949 | *** |
| Materials science | 108678 | 42869 | 0.983 | *** | 12554 | 0.834 | *** |
| Medicine | 88243 | 35598 | 0.943 | *** | 3228 | 0.601 | *** |
| Biology | 63845 | 34336 | 1.229 | *** | 3626 | 0.660 | *** |
| Computer science | 39982 | 12758 | 0.786 | *** | 1606 | 0.585 | *** |
| Mathematics | 23337 | 6169 | 0.978 | * | 1055 | 0.810 | *** |
| Physics | 23044 | 5051 | 0.883 | *** | 2417 | 0.932 | *** |
| Engineering | 19883 | 4885 | 0.766 | *** | 1027 | 0.915 | ** |
| Environmental science | 14790 | 5927 | 0.976 | ** | 1545 | 0.792 | *** |
| Geology | 9456 | 2022 | 0.925 | *** | 615 | 0.714 | *** |
| Business | 6821 | 1609 | 0.828 | *** | 139 | 0.708 | *** |
| Psychology | 5710 | 1930 | 1.036 | * | 192 | 0.719 | *** |
| Economics | 5620 | 1028 | 0.858 | *** | 132 | 0.729 | *** |
| Geography | 4924 | 1981 | 1.024 | | 211 | 0.912 | |
| Sociology | 1814 | 380 | 1.001 | | 12 | 0.807 | |
| Political science | 1267 | 317 | 1.081 | | 17 | 0.956 | |

Table S34: Statistics about the production of science and novel and atypical science in the 2010s by Japan.

| Discipline | All papers | Novel papers Count | $r_N$ | $p$-val | Atypical papers Count | $r_A$ | $p$-val |
|---|---|---|---|---|---|---|---|
| Medicine | 187272 | 70834 | 0.884 | *** | 12791 | 1.122 | *** |
| Biology | 106187 | 41845 | 0.900 | *** | 9149 | 1.002 | |
| Chemistry | 96540 | 45473 | 0.912 | *** | 12786 | 0.901 | *** |
| Materials science | 94244 | 34408 | 0.910 | *** | 12005 | 0.920 | *** |
| Physics | 29536 | 6388 | 0.871 | *** | 3049 | 0.917 | *** |
| Computer science | 24102 | 8940 | 0.914 | *** | 1433 | 0.867 | *** |
| Mathematics | 19355 | 4354 | 0.832 | *** | 968 | 0.896 | *** |
| Psychology | 14265 | 5352 | 1.150 | *** | 1115 | 1.668 | *** |
| Geology | 11752 | 2566 | 0.944 | *** | 1159 | 1.083 | ** |
| Engineering | 10699 | 3052 | 0.889 | *** | 488 | 0.809 | *** |
| Environmental science | 10435 | 3902 | 0.911 | *** | 1147 | 0.834 | *** |
| Economics | 6227 | 1058 | 0.796 | *** | 190 | 0.948 | |
| Business | 2937 | 916 | 1.095 | *** | 103 | 1.222 | * |
| Geography | 2702 | 1026 | 0.966 | | 106 | 0.838 | * |
| Sociology | 1333 | 323 | 1.157 | ** | 10 | 0.934 | |
| Political science | 1141 | 263 | 0.996 | | 19 | 1.194 | |

Table S35: Statistics about the production of novel papers in the 2010s.

| | International = 0 | | | International = 1 | | |
|---|---|---|---|---|---|---|
| Country/region | Papers | $r_N$ | $p$-val | Papers | $r_N$ | $p$-val |
| US | 1042306 | 1.007 | *** | 309223 | 1.006 | *** |
| China | 585921 | 1.035 | *** | 157721 | 1.005 | ** |
| UK | 198276 | 0.949 | *** | 104477 | 0.993 | ** |
| Japan | 188841 | 0.953 | *** | 42021 | 0.935 | *** |
| Germany | 157887 | 0.967 | *** | 77194 | 0.950 | *** |
| France | 108396 | 0.951 | *** | 54789 | 0.922 | *** |
| Canada | 118581 | 0.978 | *** | 51098 | 0.964 | *** |
| India | 188094 | 1.051 | *** | 31069 | 1.068 | *** |
| Italy | 113594 | 1.004 | * | 50892 | 0.994 | * |
| Australia | 107154 | 0.965 | *** | 52603 | 0.997 | |
| Spain | 94365 | 0.886 | *** | 42473 | 0.944 | *** |
| Korea | 146525 | 1.044 | *** | 29657 | 1.011 | ** |
| Brazil | 126150 | 1.112 | *** | 30256 | 1.110 | *** |
| Netherlands | 59623 | 1.051 | *** | 35133 | 1.046 | *** |
| Russia | 60864 | 0.797 | *** | 13652 | 0.866 | *** |
| Taiwan | 55204 | 1.000 | | 20104 | 1.090 | *** |
| Iran | 101939 | 1.085 | *** | 15765 | 1.046 | *** |
| Sweden | 37515 | 1.002 | | 22200 | 1.040 | *** |
| Turkey | 58660 | 0.980 | *** | 8363 | 0.939 | *** |
| Switzerland | 29576 | 1.009 | * | 24962 | 0.990 | * |
| Poland | 51758 | 1.027 | *** | 11940 | 0.997 | |
| Belgium | 25924 | 0.964 | *** | 19134 | 0.981 | *** |
| Israel | 23653 | 0.961 | *** | 9136 | 0.972 | *** |
| Denmark | 24493 | 1.061 | *** | 14783 | 1.059 | *** |
| Mexico | 29316 | 1.074 | *** | 12088 | 1.005 | |
| Finland | 18225 | 0.967 | *** | 10722 | 1.039 | *** |
| South Africa | 23353 | 0.930 | *** | 10768 | 1.030 | *** |
| Austria | 17700 | 1.005 | | 12582 | 1.022 | *** |
| Norway | 18654 | 0.958 | *** | 10527 | 0.976 | *** |
| Greece | 18917 | 0.962 | *** | 7986 | 0.964 | *** |
| Hong Kong | 13991 | 0.901 | *** | 12750 | 0.955 | *** |
| Portugal | 23232 | 1.038 | *** | 12473 | 1.049 | *** |
| New Zealand | 15385 | 0.947 | *** | 10026 | 0.968 | *** |
| Singapore | 15497 | 0.970 | *** | 11191 | 0.971 | *** |
| Malaysia | 26334 | 1.084 | *** | 11479 | 1.141 | *** |
| Czechia | 15923 | 0.986 | * | 7184 | 0.944 | *** |
| Egypt | 23613 | 1.165 | *** | 7754 | 1.207 | *** |
| Hungary | 10128 | 1.008 | | 4684 | 0.982 | |

* $p < 0.05$, ** $p < 0.01$, *** $p < 0.001$

Table S36: Statistics about the production of atypical papers in the 2010s.

| | International = 0 | | | International = 1 | | |
|---|---|---|---|---|---|---|
| Country/region | Papers | $r_A$ | $p$-val | Papers | $r_A$ | $p$-val |
| US | 236920 | 1.093 | *** | 82341 | 1.097 | *** |
| China | 154773 | 1.305 | *** | 47563 | 1.242 | *** |
| UK | 36724 | 0.839 | *** | 24094 | 0.938 | *** |
| Japan | 44887 | 1.081 | *** | 11654 | 1.062 | *** |
| Germany | 37573 | 1.099 | *** | 21775 | 1.097 | *** |
| France | 25175 | 1.054 | *** | 15594 | 1.075 | *** |
| Canada | 23614 | 0.930 | *** | 11926 | 0.922 | *** |
| India | 37248 | 0.994 | | 6900 | 0.971 | ** |
| Italy | 21035 | 0.888 | *** | 11544 | 0.924 | *** |
| Australia | 17766 | 0.764 | *** | 11226 | 0.872 | *** |
| Spain | 19794 | 0.887 | *** | 10620 | 0.967 | *** |
| Korea | 30436 | 1.036 | *** | 7341 | 1.025 | * |
| Brazil | 16243 | 0.684 | *** | 5270 | 0.792 | *** |
| Netherlands | 12095 | 1.018 | * | 8169 | 0.996 | |
| Russia | 10195 | 0.638 | *** | 3245 | 0.843 | *** |
| Taiwan | 11874 | 1.027 | ** | 4167 | 0.926 | *** |
| Iran | 17748 | 0.902 | *** | 2979 | 0.810 | *** |
| Sweden | 7006 | 0.894 | *** | 5187 | 0.995 | |
| Turkey | 9162 | 0.731 | *** | 1606 | 0.738 | *** |
| Switzerland | 7260 | 1.182 | *** | 6723 | 1.092 | *** |
| Poland | 7681 | 0.728 | *** | 2344 | 0.802 | *** |
| Belgium | 5527 | 0.981 | | 4614 | 0.969 | * |
| Israel | 4763 | 0.924 | *** | 2209 | 0.963 | * |
| Denmark | 4677 | 0.968 | ** | 3459 | 1.015 | |
| Mexico | 4553 | 0.797 | *** | 2384 | 0.812 | *** |
| Finland | 3438 | 0.871 | *** | 2528 | 1.003 | |
| South Africa | 2748 | 0.523 | *** | 1886 | 0.739 | *** |
| Austria | 3539 | 0.959 | ** | 3013 | 1.003 | |
| Norway | 3140 | 0.770 | *** | 2206 | 0.838 | *** |
| Greece | 3451 | 0.838 | *** | 1630 | 0.806 | *** |
| Hong Kong | 3154 | 0.970 | * | 3485 | 1.069 | *** |
| Portugal | 3881 | 0.828 | *** | 2589 | 0.892 | *** |
| New Zealand | 2694 | 0.792 | *** | 2197 | 0.868 | *** |
| Singapore | 4230 | 1.264 | *** | 3193 | 1.135 | *** |
| Malaysia | 3590 | 0.706 | *** | 1938 | 0.789 | *** |
| Czechia | 2911 | 0.861 | *** | 1726 | 0.929 | *** |
| Egypt | 2987 | 0.704 | *** | 1242 | 0.792 | *** |
| Hungary | 1768 | 0.840 | *** | 963 | 0.827 | *** |

* $p < 0.05$, ** $p < 0.01$, *** $p < 0.001$
